# Supplementary material for: Using SIMD and SIMT vectorization to evaluate sparse chemical kinetic Jacobian matrices and thermochemical source terms
Source: arXiv:1809.01029 ancillary file (2018-09-04)
Supplement: Supplementary file 1 [file derivations.pdf]

# Supplemental: A System of Equations and Derivation of Sparse Constant-Pressure/Constant-Volume Chemical Kinetic Jacobians for `pyJac`

Nicholas Curtis<sup>a,\*</sup>, Kyle E. Niemeyer<sup>b</sup>, Chih-Jen Sung<sup>a</sup>

<sup>a</sup>*Department of Mechanical Engineering, University of Connecticut, Storrs, CT 06269, USA*

<sup>b</sup>*School of Mechanical, Industrial, and Manufacturing Engineering, Oregon State University, Corvallis, OR 97331, USA*

---

## Abstract

This document supplements the work, *Using SIMD and SIMT vectorization to evaluate sparse chemical kinetic Jacobian matrices and thermochemical source terms* and presents the system of chemical kinetic equations evaluated by the new version of code-generation platform, `pyJac-v2`. First, the thermochemical source terms for fixed-mass, adiabatic constant-pressure/constant-volume (CONP/CONV) reactors are given, followed by the derivation of the sparse analytical chemical kinetic Jacobian for both reactors. Finally, the resulting Jacobian equations are summarized using a generalized notation for a quick-reference.

---

## 1. Introduction

This document is a supplement to the paper—*Using SIMD and SIMT vectorization to evaluate sparse chemical kinetic Jacobian matrices and thermochemical source terms*—and is provided as a reference guide to the equations evaluated by `pyJac v2.0`, a code-generation platform for the evaluation of chemical source terms and analytical chemical kinetic Jacobians of constant-pressure/constant-volume, fixed-mass, adiabatic reactors. Note that equations specific to the constant-pressure or constant-volume derivation will be marked with CONP or CONV respectively. The derivations in this document

---

\*Corresponding author

based upon the output of the script [derivations.py](#) in the GitHub repository for this paper. This script depends on the symbolic mathematics library SymPy [1], and was tested with versions 1.0 and 1.1.1

## 2. Governing equations

### 2.1. State variables

The state vector for this derivation consists of the temperature, a thermodynamic state parameter (pressure or volume) and the number of moles of all species except the last in the model:

$$\Phi = \{T, V, n_1, n_2 \dots n_{N_{\text{sp}}-1}\} \quad \text{for CONP}, \quad (1a)$$

$$\Phi = \{T, P, n_1, n_2 \dots n_{N_{\text{sp}}-1}\} \quad \text{for CONV}, \quad (1b)$$

where  $T$  is the temperature,  $V$  and  $P$  the volume and pressure respectively, and  $n_j$  the number of moles of the  $j$ th species in the model (containing  $N_{\text{sp}}$  total species).

From the ideal gas law, the number of moles of the final species is determined as:

$$\begin{aligned} n &= \frac{VP}{T\mathcal{R}} = \sum_{i=1}^{N_{\text{sp}}} n_i, \\ n_{N_{\text{sp}}} &= \frac{VP}{T\mathcal{R}} - \sum_{i=1}^{N_{\text{sp}}-1} n_i, \end{aligned} \quad (2)$$

where  $\mathcal{R}$  is the ideal gas constant in molar units.

### 2.2. Thermo-chemical source terms

The evolution of the thermo-chemical state variables of this system is described by a set of ordinary-differential equations:

$$f = \frac{d\Phi}{dt} = \left\{ \frac{dT}{dt}, \frac{dV}{dt}, \frac{dn_1}{dt}, \frac{dn_2}{dt} \dots \frac{dn_{N_{\text{sp}}-1}}{dt} \right\} \quad \text{for CONP}, \quad (3a)$$

$$f = \frac{d\Phi}{dt} = \left\{ \frac{dT}{dt}, \frac{dP}{dt}, \frac{dn_1}{dt}, \frac{dn_2}{dt} \dots \frac{dn_{N_{\text{sp}}-1}}{dt} \right\} \quad \text{for CONV}. \quad (3b)$$

For both CONP and CONV, the molar source terms are [2]:

$$\frac{dn_k}{dt} = V\dot{\omega}_k \quad k = 1, \dots, N_{\text{sp}} - 1, \quad (4)$$

where  $\dot{\omega}_k$  is the  $k$ th species' overall production rate, and the temperature production rate [2] is:

$$\frac{dT}{dt} = -\frac{\sum_{k=1}^{N_{\text{sp}}} H_k \dot{\omega}_k}{\sum_{k=1}^{N_{\text{sp}}} [C]_k C_{p,k}} \quad \text{for CONP,} \quad (5a)$$

$$\frac{dT}{dt} = -\frac{\sum_{k=1}^{N_{\text{sp}}} U_k \dot{\omega}_k}{\sum_{k=1}^{N_{\text{sp}}} [C]_k C_{v,k}} \quad \text{for CONV,} \quad (5b)$$

where  $H_k$ ,  $U_k$ ,  $C_{p,k}$  and  $C_{v,k}$  are the enthalpy, internal energy, constant-pressure and constant-volume specific heat of species  $k$  in molar units respectively, while  $[C]_k$  is the concentration, given by:

$$[C]_k = \frac{n_k}{V}. \quad (6)$$

From the ideal gas law, source terms for the volume and pressure variables may derived:

$$\frac{dV}{dt} = \frac{\mathcal{R}}{P} \left( T \frac{dn}{dt} + \frac{dT}{dt} n \right) \quad \text{for CONP,} \quad (7a)$$

$$\frac{dP}{dt} = \frac{\mathcal{R}}{V} \left( T \frac{dn}{dt} + \frac{dT}{dt} n \right) \quad \text{for CONV.} \quad (7b)$$

To determine  $\frac{dn}{dt}$ , conservation of mass is invoked:

$$\frac{dm}{dt} = 0 = \sum_{k=1}^{N_{\text{sp}}} W_k \frac{dn_k}{dt}, \quad (8)$$

where  $W_k$  is the molecular weight of the  $k$ th species. From Eq. (8), the source term of the last species may be written in terms of the species included in the state vector:

$$\frac{dn_{N_{\text{sp}}}}{dt} = -\sum_{k=1}^{N_{\text{sp}}-1} \frac{W_k}{W_{N_{\text{sp}}}} \frac{dn_k}{dt} \quad (9)$$

Using Eq. (9), the total molar rate of change can be determined:

$$\frac{dn}{dt} = \sum_{k=1}^{N_{\text{sp}}} \frac{dn_k}{dt},$$

$$\frac{dn}{dt} = \sum_{k=1}^{N_{\text{sp}}-1} \left(1 - \frac{W_k}{W_{N_{\text{sp}}}}\right) \frac{dn_k}{dt} \quad (10)$$

Combining Eqs. (4), (7) and (10) gives the final form of the pressure and volume terms:

$$\frac{dV}{dt} = V \left( \frac{T\mathcal{R}}{P} \sum_{k=1}^{N_{\text{sp}}-1} \left(1 - \frac{W_k}{W_{N_{\text{sp}}}}\right) \dot{\omega}_k + \frac{1}{T} \frac{dT}{dt} \right) \quad \text{for CONP}, \quad (11a)$$

$$\frac{dP}{dt} = T\mathcal{R} \sum_{k=1}^{N_{\text{sp}}-1} \left(1 - \frac{W_k}{W_{N_{\text{sp}}}}\right) \dot{\omega}_k + \frac{P}{T} \frac{dT}{dt} \quad \text{for CONV}. \quad (11b)$$

$W_k$  and  $W_{N_{\text{sp}}}$  are the molecular weights of species  $k$  and  $N_{\text{sp}}$ , respectively.

Additionally, the concentration and moles of the last species in the model (which is not a state variable) may be expanded in terms of the state variables of the system:

$$[C]_{N_{\text{sp}}} = [C] - \sum_{k=1}^{N_{\text{sp}}-1} [C]_k, \quad (12)$$

where  $[C]$  is the total concentration:

$$[C] = \frac{P}{T\mathcal{R}}. \quad (13)$$

Using Eqs. (4), (9) and (12), the temperature source terms may be expanded to contain only state variables (i.e., by removal of the last species' source term and overall production rate):

$$\frac{dT}{dt} = - \frac{\sum_{k=1}^{N_{\text{sp}}-1} \left( H_k - \frac{W_k H_{N_{\text{sp}}}}{W_{N_{\text{sp}}}} \right) \dot{\omega}_k}{[C]C_{p,N_{\text{sp}}} + \sum_{k=1}^{N_{\text{sp}}-1} \left( C_{p,k} - C_{p,N_{\text{sp}}} \right) [C]_k} \quad \text{for CONP}, \quad (14a)$$

$$\frac{dT}{dt} = - \frac{\sum_{k=1}^{N_{\text{sp}}-1} \left( U_k - \frac{W_k U_{N_{\text{sp}}}}{W_{N_{\text{sp}}}} \right) \dot{\omega}_k}{[C]C_{v,N_{\text{sp}}} + \sum_{k=1}^{N_{\text{sp}}-1} \left( C_{v,k} - C_{v,N_{\text{sp}}} \right) [C]_k} \quad \text{for CONV}. \quad (14b)$$

This form of the temperature source term will be used for derivation of Jacobian terms, but Eq. (5) will often be used as well due to its compactness.

### 2.3. Thermal properties

The standard-state thermodynamic properties (in molar units) for a gaseous species  $k$  is defined using the standard seven-coefficient polynomial of Gordon and McBride [3]:

$$\frac{C_{p,k}^\circ}{\mathcal{R}} = a_{0,k} + T(a_{1,k} + T(a_{2,k} + T(a_{3,k} + a_{4,k}T))) , \quad (15)$$

$$\frac{H_k^\circ}{\mathcal{R}} = T \left( a_{0,k} + T \left( \frac{a_{1,k}}{2} + T \left( \frac{a_{2,k}}{3} + T \left( \frac{a_{3,k}}{4} + \frac{a_{4,k}}{5} T \right) \right) \right) \right) + a_{5,k} , \quad (16)$$

$$\frac{S_k^\circ}{\mathcal{R}} = a_{0,k} \ln T + T \left( a_{1,k} + T \left( \frac{a_{2,k}}{2} + T \left( \frac{a_{3,k}}{3} + \frac{a_{4,k}}{4} T \right) \right) \right) + a_{6,k} , \quad (17)$$

where  $C_{p,k}$  and  $H_k$  are as described previously,  $S_k$  is the entropy in molar units, and the  $^\circ$  indicates a standard-state property at one atmosphere (equivalent to the property at any pressure for calorically perfect gases).

### 2.4. Reaction rate expressions

The net species production rate for species  $k$  is defined as:

$$\dot{\omega}_k = \sum_{i=1}^{N_{\text{reac}}} \nu_{k,i} q_i , \quad (18)$$

where  $N_{\text{reac}}$  is the number of reactions in the chemical kinetic model,  $\nu_{k,i}$  the overall stoichiometric coefficient of species  $k$  in reaction  $i$  and  $q_i$  the net rate-of-progress for reaction  $i$ :

$$\nu_{k,i} = \nu''_{k,i} - \nu'_{k,i} , \quad (19)$$

$$q_i = R_i c_i , \quad (20)$$

with  $\nu''_{k,i}$  and  $\nu'_{k,i}$  the product and reactant stoichiometric coefficients (respectively) of species  $k$  in reaction  $i$ . The base rate-of-progress for the  $i$ th reversible reaction  $R_i$  is given by:

$$R_i = R_{f,i} - R_{r,i} , \quad (21)$$

$$R_{f,i} = k_{f,i} \prod_{k=1}^{N_{\text{sp}}} [C]_k^{\nu'_{k,i}} , \quad (22)$$

$$R_{r,i} = k_{r,i} \prod_{k=1}^{N_{\text{sp}}} [C]_k^{\nu''_{k,i}} , \quad (23)$$

where  $k_{f,i}$  and  $k_{r,i}$  are the forward and reverse reaction coefficients (respectively) for the  $i$ th reaction, and the third-body/pressure modification  $c_i$  is given by:

$$c_i = \begin{cases} 1 & \text{for elementary reactions,} \\ [X]_i & \text{for third-body enhanced reactions,} \\ \frac{P_{r,i}}{1 + P_{r,i}} F_i & \text{for unimolecular/ recombination fall-off reactions, and} \\ \frac{1}{1 + P_{r,i}} F_i & \text{for chemically-activated bimolecular reactions,} \end{cases} \quad (24)$$

where for the  $i$ th reaction  $[X]_i$  is the third-body concentration,  $P_{r,i}$  is the reduced pressure, and  $F_i$  is the falloff blending factor. These terms are defined in the following sections.

The forward reaction rate coefficient  $k_{f,i}$  is given by the three-parameter Arrhenius expression:

$$k_{f,i} = A_i T^{\beta_i} \exp\left(-\frac{E_{a,i}}{T\mathcal{R}}\right), \quad (25)$$

where  $A_i$  is the pre-exponential factor,  $\beta_i$  is the temperature exponent, and  $T_{a,i}$  is the activation temperature given by  $T_{a,i} = E_{a,i}/\mathcal{R}$ .

As given by Lu and Law [4], depending on the value of the Arrhenius parameters,  $k_{f,i}$  can be calculated in different ways to minimize the computational cost:

$$k_{f,i} = \begin{cases} A_i & \text{if } \beta = 0 \text{ and } T_{a,i} = 0, \\ \exp(\log A_i + \beta_i \log T) & \text{if } \beta_i \neq 0 \text{ and } T_{a,i} = 0, \\ \exp(\log A_i + \beta_i \log T - T_{a,i}/T) & \text{if } \beta_i \neq 0 \text{ and } T_{a,i} \neq 0, \\ \exp(\log A_i - T_{a,i}/T) & \text{if } \beta_i = 0 \text{ and } T_{a,i} \neq 0, \text{ and} \\ A_i \prod^{\beta_i} T & \text{if } T_{a,i} = 0 \text{ and } \beta_i \in \mathbb{Z}, \end{cases} \quad (26)$$

where  $\mathbb{Z}$  is the set of integers; the extent of this specialization can be controlled when generating code via `pyjac`.

### 2.5. Reverse rate coefficient

By definition, the reverse rate coefficient,  $k_{r,i}$ , of irreversible reactions is zero, while reversible reactions may have non-zero  $k_{r,i}$ . Note that in `pyJac`,

reversible reactions with explicit reverse Arrhenius parameters are split into two irreversible reactions; this simplifies calculation inside the generated code, and eases comparison to Cantera [5] which applies the same transformation. For reversible reactions without an explicit parameterization, the reverse rate coefficient is calculated from ratio of the forward rate coefficient and the equilibrium constant:

$$k_{r,i} = \frac{k_{f,i}}{K_{c,i}} , \quad (27)$$

$$K_{c,i} = K_{p,i} \left( \frac{P_{atm}}{T\mathcal{R}} \right)^{\sum_{k=1}^{N_{sp}} \nu_{k,i}} , \text{ and} \quad (28)$$

$$K_{p,i} = \exp \left( \frac{\Delta S_i^\circ}{\mathcal{R}} - \frac{\Delta H_i^\circ}{\mathcal{R}T} \right) = \exp \left( \sum_{k=1}^{N_{sp}} \nu_{ki} \left( \frac{S_k^\circ}{\mathcal{R}} - \frac{H_k^\circ}{\mathcal{R}T} \right) \right) , \quad (29)$$

where  $P_{atm}$  is the pressure of one standard atmosphere in appropriate units.

By combining Eqs. (28) and (29), we obtain:

$$K_{c,i} = \left( \left( \frac{P_{atm}}{\mathcal{R}} \right)^{\sum_{k=1}^{N_{sp}} \nu_{k,i}} \right) \exp \left( \sum_{k=1}^{N_{sp}} \nu_{k,i} B_k \right) , \quad (30)$$

where from Eqs. (16) and (17),  $B_k$  is:

$$\begin{aligned} B_k &= \frac{S_k^\circ}{\mathcal{R}} - \frac{H_k^\circ}{\mathcal{R}T} - \ln T , \\ B_k &= T \left( T \left( T \left( \frac{Ta_{k,4}}{20} + \frac{a_{k,3}}{12} \right) + \frac{a_{k,2}}{6} \right) + \frac{a_{k,1}}{2} \right) \\ &\quad + (a_{k,0} - 1) \log(T) - a_{k,0} + a_{k,6} - \frac{a_{k,5}}{T} . \end{aligned} \quad (31)$$

## 2.6. Third-body effects

For a reaction enhanced (or diminished) by the presence of a third body, the reaction rate is modified by the third-body concentration  $[X]_i$  given by:

$$[X]_i = \sum_{k=1}^{N_{sp}} \alpha_{k,i} [C]_k , \quad (32)$$

where  $\alpha_{k,i}$  is the third-body efficiency of species  $k$  in the  $i$ th reaction. For a default third-body efficiency of  $\alpha_{k,i} = 1$ , this may be rearranged to the

compact-storage form:

$$[X]_i = [C] + \sum_{k=1}^{N_{\text{sp}}} (\alpha_{k,i} - 1) [C]_k , \quad (33)$$

where only species with non-default third-body efficiencies must be stored in the model. Expanding the concentration of the last species gives:

$$[X]_i = [C] \alpha_{N_{\text{sp}},i} + \sum_{k=1}^{N_{\text{sp}}-1} (-\alpha_{N_{\text{sp}},i} + \alpha_{k,i}) [C]_k . \quad (34)$$

This form will be denoted as the mixture-based (or **mix** for short) third-body efficiency.

If all species in the mixture contribute equally as third bodies, i.e.,  $\alpha_{k,i} = 1$  for all species, then:

$$[X]_i = [C] = \frac{P}{RT} . \quad (35)$$

This form will be called the **unity**-based third-body efficiency.

In addition, a single species may act as the third body in which case

$$[X]_i = [C]_m , \quad (36)$$

where the  $m$ th species is the third body. For evaluation of Jacobian entries, the expanded form:

$$[X]_i = \left( [C] - \sum_{k=1}^{N_{\text{sp}}-1} [C]_k \right) \delta_{N_{\text{sp}},m} + (-\delta_{N_{\text{sp}},m} + 1) [C]_m \quad (37)$$

will be used, where the Kronecker delta  $\delta_{N_{\text{sp}},m}$  is unity if and only if the third body species  $m$  is the last species in the model. Equation (37) will be referred to as the **species**-based third-body efficiency.

## 2.7. Falloff and chemically-activated reactions

Unlike elementary and third-body reactions, falloff/chemically-activated reactions exhibit a pressure dependence described as a blending of rates at low- and high-pressure limits; thus, the rate coefficients depend on a mixture of low-pressure ( $k_{0,i}$ ) and high-pressure-limit ( $k_{\infty,i}$ ) coefficients, each with corresponding Arrhenius parameters and expressed using Eq. (25). It is noted that when the forward rate coefficient is used—e.g., as in Eq. (22)— $k_{f,i}$



is taken to be the high-pressure reaction coefficient ( $k_{\infty,i}$ ) for falloff reactions and the low-pressure reaction coefficient ( $k_{0,i}$ ) for chemically-activated reactions [5]. The ratio of the coefficients  $k_{0,i}$  and  $k_{\infty,i}$ , combined with the third-body concentration, define a reduced pressure  $P_{r,i}$  given by

$$P_{r,i} = \frac{[X]_i k_{0,i}}{k_{\infty,i}} \quad (38)$$

where  $[X]_i$  is the appropriate third-body concentration as described in Section 2.6.

The falloff blending factor  $F_i$  used in Eq. (24) is determined based on one of three representations: the Lindemann [6], Troe [7], and SRI [8] falloff approaches

$$F_i = \begin{cases} 1 & \text{for Lindemann,} \\ F_{\text{cent}}^{(1+(A_{\text{Troe}}/B_{\text{Troe}})^2)^{-1}} & \text{for Troe, or} \\ dT^e \left( a \cdot \exp\left(-\frac{b}{T}\right) + \exp\left(-\frac{T}{c}\right) \right)^X & \text{for SRI.} \end{cases} \quad (39)$$

The Troe representation is described by the variables:

$$F_{\text{cent}} = a \exp\left(-\frac{T}{T^*}\right) + (-a + 1) \exp\left(-\frac{T}{T^{***}}\right) + \exp\left(-\frac{T^{**}}{T}\right), \quad (40)$$

$$A_{\text{Troe}} = -0.67 \log_{10}(F_{\text{cent}}) + \log_{10}(P_{r,i}) - 0.4, \text{ and} \quad (41)$$

$$B_{\text{Troe}} = -1.1762 \log_{10}(F_{\text{cent}}) - 0.14 \log_{10}(P_{r,i}) + 0.806, \quad (42)$$

where  $a$ ,  $T^{***}$ ,  $T^*$ , and  $T^{**}$  are specified parameters. The final parameter  $T^{**}$  is optional, and, if it is not used, the final term of  $F_{\text{cent}}$  is omitted.

The exponent used in the SRI representation is given by:

$$X = \frac{1}{\log_{10}^2(P_{r,i}) + 1}. \quad (43)$$

The parameters  $a$ ,  $b$ , and  $c$  in the SRI falloff blending factor are required while  $d$  and  $e$  are optional; if not specified,  $d = 1$  and  $e = 0$ .

## 2.8. Pressure-dependent reactions

In addition to the falloff approach given previously, two additional formulations can be used to describe the pressure dependence of reactions that do

not follow the modification factor  $c_i$  approach. The first involves logarithmic interpolation between Arrhenius rates at two pressures [5, 9] (often termed P-Log reactions), each evaluated using Eq. (25):

$$k_1(T) = A_1 T^{\beta_1} \exp\left(-\frac{T_{a,1}}{T}\right) \text{ at } P_1 \text{ and,} \quad (44)$$

$$k_2(T) = A_2 T^{\beta_2} \exp\left(-\frac{T_{a,2}}{T}\right) \text{ at } P_2, \quad (45)$$

where the Arrhenius coefficients are given for each pressure  $P_1$  and  $P_2$ . Then, the reaction rate coefficient at a particular pressure  $P$  between  $P_1$  and  $P_2$  can be determined through logarithmic interpolation:

$$\log(k_{f,i}) = \frac{(-\log(k_1) + \log(k_2))(-\log(P_1) + \log(P))}{-\log(P_1) + \log(P_2)} + \log(k_1) \quad (46)$$

In addition, the pressure dependence of a reaction can be expressed through a bivariate Chebyshev polynomial fit [5, 9–12]:

$$\log_{10} k_f(T, P) = \sum_{i=1}^{N_T} \sum_{j=1}^{N_p} \eta_{ij} \phi_i(\tilde{T}) \phi_j(\tilde{P}), \quad (47)$$

where  $\eta_{ij}$  is the coefficient corresponding to the grid points  $i$  and  $j$ ,  $N_T$  and  $N_p$  are the numbers of grid points for temperature and pressure, respectively, and  $\phi_n$  is the Chebyshev polynomial of the first kind of degree  $n-1$  typically expressed as

$$\phi_n(x) = \mathcal{T}_{n-1}(x) = \cos((n-1) \arccos(x)) \quad \text{for } |x| \leq 1. \quad (48)$$

The reduced temperature  $\tilde{T}$  and pressure  $\tilde{P}$  are given by

$$\tilde{T} \equiv \frac{2T^{-1} - T_{\min}^{-1} - T_{\max}^{-1}}{T_{\max}^{-1} - T_{\min}^{-1}} \quad \text{and,} \quad (49)$$

$$\tilde{P} \equiv \frac{2 \log_{10} P - \log_{10} P_{\min} - \log_{10} P_{\max}}{\log_{10} P_{\max} - \log_{10} P_{\min}}, \quad (50)$$

where  $T_{\min} \leq T \leq T_{\max}$  and  $P_{\min} \leq P \leq P_{\max}$  describe the ranges of validity for temperature and pressure.

### 3. Jacobian derivation

Let  $\mathcal{J}$  denote the Jacobian matrix corresponding to the set of ODEs defined in Eq. (3).  $\mathcal{J}$  is filled with the partial derivatives  $\partial f/\partial\Phi$ , such that:

$$\mathcal{J}_{i,j} = \frac{\partial f_i}{\partial \Phi_j}, \quad i, j = 1 \dots N_{\text{sp}} + 1. \quad (51)$$

where  $i$  and  $j$  correspond to the row and column, respectively, of the entry in the Jacobian matrix. The Jacobian entries resulting from Eq. (51) are derived in Sections 3.1 to 3.3, while various subcomponents of the Jacobian are derived in Sections 3.5.1 to 3.5.4 and 3.6. The final form of the Jacobian can be found in Section 4, which provides a useful summary for this document.

We note that some parts of the Jacobian derivation—in particular derivatives of the energy equation—are quite complicated. The aim of this document is to provide the reader with an overview of the derivation process; some intermediate steps are left out due to length and typesetting constraints. For a complete derivation, the reader is directed to the output of the [derivations.py](#) script, from which this document was compiled.

#### 3.1. Temperature source term derivatives

##### 3.1.1. Temperature derivative

First, the temperature source term's derivative with respect to the temperature:

$$\mathcal{J}_{1,1} = \frac{\partial}{\partial T} \frac{dT}{dt},$$

or more simply:

$$\mathcal{J}_{1,1} = \frac{\partial \dot{T}}{\partial T}, \quad (52)$$

will be derived. As the derivation process for this Jacobian entry is very similar between CONP and CONV energy equations, we will focus on the Jacobian entry for the CONP temperature source term and give the result for CONV at the end of this section.

The derivative of a species concentration with respect to temperature for both CONP and CONV is:

$$\frac{\partial [C]_k}{\partial T} = \begin{cases} \frac{\partial}{\partial T} \left( \frac{n_k}{V} \right) = 0 & \text{for } k \neq N_{\text{sp}} \text{ and,} \\ \frac{\partial}{\partial T} \left( [C] - \sum_{k=1}^{N_{\text{sp}}-1} \frac{n_k}{V} \right) = -\frac{[C]}{T} & \text{for } k = N_{\text{sp}}, \end{cases} \quad (53)$$

as the pressure and volume are either constants (for CONP and CONV respectively) or a state variable that is a function of time only.

Next, the derivative of full form of the temperature source term Eq. (14) with respect to temperature will be considered. To make the result more manageable, the denominator of Eq. (14) is first collapsed back into the form of Eq. (5), yielding for CONP:

$$\begin{aligned} \frac{\partial \dot{T}}{\partial T} = & - \frac{\left( [C] \left( \frac{C_{p,N_{\text{sp}}}}{T} - \frac{dC_{p,N_{\text{sp}}}}{dT} \right) - \sum_{k=1}^{-1+N_{\text{sp}}} \left( -\frac{dC_{p,N_{\text{sp}}}}{dT} + \frac{dC_{p,k}}{dT} \right) [C]_k \right)}{\left( \sum_{k=1}^{N_{\text{sp}}} [C]_k C_{p,k} \right)^2} \times \\ & \sum_{k=1}^{-1+N_{\text{sp}}} \left( H_k - \frac{W_k H_{N_{\text{sp}}}}{W_{N_{\text{sp}}}} \right) \dot{\omega}_k - \\ & \frac{\sum_{k=1}^{-1+N_{\text{sp}}} \left( \left( H_k - \frac{W_k H_{N_{\text{sp}}}}{W_{N_{\text{sp}}}} \right) \frac{\partial \dot{\omega}_k}{\partial T} + \left( \frac{dH_k}{dT} - \frac{W_k}{W_{N_{\text{sp}}}} \frac{dH_{N_{\text{sp}}}}{dT} \right) \dot{\omega}_k \right)}{\sum_{k=1}^{N_{\text{sp}}} [C]_k C_{p,k}}. \end{aligned} \quad (54)$$

Next, Eq. (5) may be factored out, yielding:

$$\begin{aligned} \frac{\partial \dot{T}}{\partial T} = & \frac{1}{\sum_{k=1}^{N_{\text{sp}}} [C]_k C_{p,k}} \left[ \frac{dT}{dt} \times \right. \\ & \left( [C] \left( \frac{C_{p,N_{\text{sp}}}}{T} - \frac{dC_{p,N_{\text{sp}}}}{dT} \right) - \sum_{k=1}^{-1+N_{\text{sp}}} \left( -\frac{dC_{p,N_{\text{sp}}}}{dT} + \frac{dC_{p,k}}{dT} \right) [C]_k \right) - \\ & \left. \sum_{k=1}^{-1+N_{\text{sp}}} \left( \left( H_k - \frac{W_k H_{N_{\text{sp}}}}{W_{N_{\text{sp}}}} \right) \frac{\partial \dot{\omega}_k}{\partial T} + \left( \frac{dH_k}{dT} - \frac{W_k}{W_{N_{\text{sp}}}} \frac{dH_{N_{\text{sp}}}}{dT} \right) \dot{\omega}_k \right) \right]. \end{aligned} \quad (55)$$

Now, the identity:

$$[C] = \sum_{k=1}^{N_{\text{sp}}} [C]_k \quad (56)$$

is invoked to simplify the specific heat terms:

$$\begin{aligned} \frac{\partial \dot{T}}{\partial T} = & \frac{1}{\sum_{k=1}^{N_{\text{sp}}} [C]_k C_{p,k}} \left[ \frac{dT}{dt} \sum_{k=1}^{N_{\text{sp}}} \left( -\frac{dC_{p,k}}{dT} + \frac{C_{p,N_{\text{sp}}}}{T} \right) [C]_k + \right. \\ & \left. \sum_{k=1}^{-1+N_{\text{sp}}} \left( \left( -H_k + \frac{W_k H_{N_{\text{sp}}}}{W_{N_{\text{sp}}}} \right) \frac{\partial \dot{\omega}_k}{\partial T} + \right. \right. \end{aligned}$$

$$\left( -\frac{dH_k}{dT} + \frac{W_k}{W_{N_{\text{sp}}}} \frac{dH_{N_{\text{sp}}}}{dT} \right) \dot{\omega}_k \Bigg] . \quad (57)$$

Finally, the derivative of species enthalpy with respect to temperature:

$$C_{p,k} = \frac{dH_k}{dT} , \quad (58)$$

is substituted in, giving:

$$\begin{aligned} \frac{\partial \dot{T}}{\partial T} = & \frac{1}{\sum_{k=1}^{N_{\text{sp}}} [C]_k C_{p,k}} \left[ \frac{dT}{dt} \sum_{k=1}^{N_{\text{sp}}} \left( -\frac{dC_{p,k}}{dT} + \frac{C_{p,N_{\text{sp}}}}{T} \right) [C]_k + \right. \\ & \sum_{k=1}^{-1+N_{\text{sp}}} \left( \left( -H_k + \frac{W_k H_{N_{\text{sp}}}}{W_{N_{\text{sp}}}} \right) \frac{\partial \dot{\omega}_k}{\partial T} + \right. \\ & \left. \left. \left( -C_{p,k} + \frac{W_k C_{p,k}}{W_{N_{\text{sp}}}} \right) \dot{\omega}_k \right) \right] \quad \text{for CONP, } (59a) \end{aligned}$$

and similarly:

$$\begin{aligned} \frac{\partial \dot{T}}{\partial T} = & \frac{1}{\sum_{k=1}^{N_{\text{sp}}} [C]_k C_{v,k}} \left[ \frac{dT}{dt} \sum_{k=1}^{N_{\text{sp}}} \left( -\frac{dC_{v,k}}{dT} + \frac{C_{v,N_{\text{sp}}}}{T} \right) [C]_k + \right. \\ & \sum_{k=1}^{-1+N_{\text{sp}}} \left( \left( -U_k + \frac{W_k U_{N_{\text{sp}}}}{W_{N_{\text{sp}}}} \right) \frac{\partial \dot{\omega}_k}{\partial T} + \right. \\ & \left. \left. \left( -C_{v,k} + \frac{W_k C_{v,N_{\text{sp}}}}{W_{N_{\text{sp}}}} \right) \dot{\omega}_k \right) \right] \quad \text{for CONV. } (59b) \end{aligned}$$

The species production rate derivative with respect to temperature will be defined in Section 3.4.

### 3.1.2. State parameter derivatives

Next, the derivative of the energy equation with respect to the thermodynamic state parameter will be considered:

$$\mathcal{J}_{1,2} = \frac{\partial \dot{T}}{\partial V} \quad \text{for CONP,} \quad (60a)$$

$$\mathcal{J}_{1,2} = \frac{\partial \dot{T}}{\partial P} \quad \text{for CONV.} \quad (60b)$$

First, the derivative of the concentration of a species  $k$  with respect to the state parameter is:

$$\frac{\partial [C]_k}{\partial V} = \begin{cases} -\frac{[C]_k}{V} & \text{with } k \neq N_{\text{sp}} \\ \frac{1}{V} \sum_{k=1}^{N_{\text{sp}}-1} [C]_k & \text{with } k = N_{\text{sp}} \end{cases} \quad \text{for CONP,} \quad (61a)$$

$$\frac{\partial [C]_k}{\partial P} = \begin{cases} 0 & \text{with } k \neq N_{\text{sp}} \\ \frac{1}{T\mathcal{R}} & \text{with } k = N_{\text{sp}} \end{cases} \quad \text{for CONV,} \quad (61b)$$

while the specific heat and enthalpy/internal-energy are independent of the state parameter for both CONP and CONV. Following the same procedure as in Section 3.1.1, the result of Eq. (60) is simplified by collapsing the specific-heat/concentration sum, and substituting in the temperature source term, giving:

$$\frac{\partial \dot{T}}{\partial V} = \frac{1}{\sum_{k=1}^{N_{\text{sp}}} [C]_k C_{p,k}} \left[ -\sum_{k=1}^{-1+N_{\text{sp}}} \left( H_k - \frac{W_k H_{N_{\text{sp}}}}{W_{N_{\text{sp}}}} \right) \frac{\partial \dot{\omega}_k}{\partial V} + \frac{1}{V} \frac{dT}{dt} \sum_{k=1}^{-1+N_{\text{sp}}} \left( -C_{p,N_{\text{sp}}} + C_{p,k} \right) [C]_k \right] \quad \text{for CONP,} \quad (62a)$$

$$\frac{\partial \dot{T}}{\partial P} = \frac{1}{\sum_{k=1}^{N_{\text{sp}}} [C]_k C_{v,k}} \left[ -\sum_{k=1}^{-1+N_{\text{sp}}} \left( U_k - \frac{W_k U_{N_{\text{sp}}}}{W_{N_{\text{sp}}}} \right) \frac{\partial \dot{\omega}_k}{\partial P} - \frac{C_{v,N_{\text{sp}}}}{T\mathcal{R}} \frac{dT}{dt} \right] \quad \text{for CONV.} \quad (62b)$$

The derivative of the species production rate with respect to the state parameter will be computed in Section 3.4.

### 3.1.3. Molar derivative

Finally, the derivative of the temperature source term with respect to the moles of species  $j$  is:

$$\mathcal{J}_{1,j+2} = \frac{\partial \dot{T}}{\partial n_j} \quad (63)$$

First, the molar derivative of a species concentration is computed as:

$$\frac{\partial [C]_k}{\partial n_j} = \begin{cases} \frac{\delta_{jk}}{V} & \text{for } k \neq N_{\text{sp}} \\ -\frac{1}{V} & \text{for } k = N_{\text{sp}} \end{cases} \quad (64)$$

Or put succinctly:

$$\frac{\partial [C]_k}{\partial n_j} = \frac{\delta_{jk} - \delta_{N_{\text{sp}}k}}{V} \quad (65)$$

The derivative of the energy equation with respect to the moles of species  $j$ —after collapsing the specific-heat/ concentration sum, as in Similar to Section 3.1.1—is given by:

$$\begin{aligned} \frac{\partial \dot{T}}{\partial n_j} = & \frac{\left( \sum_{k=1}^{-1+N_{\text{sp}}} \left( H_k - \frac{W_k H_{N_{\text{sp}}}}{W_{N_{\text{sp}}}} \right) \dot{\omega}_k \right) \sum_{k=1}^{-1+N_{\text{sp}}} - \frac{\delta_{jk}}{V} (C_{p,N_{\text{sp}}} - C_{p,k})}{\left( \sum_{k=1}^{N_{\text{sp}}} [C]_k C_{p,k} \right)^2} \\ & - \frac{1}{\sum_{k=1}^{N_{\text{sp}}} [C]_k C_{p,k}} \sum_{k=1}^{-1+N_{\text{sp}}} \left( H_k - \frac{W_k H_{N_{\text{sp}}}}{W_{N_{\text{sp}}}} \right) \frac{\partial \dot{\omega}_k}{\partial n_j}. \end{aligned} \quad (66)$$

Next, the Kronecker delta summation is simplified, and the compact form of the energy equation (Eq. (5)) factored out yielding:

$$\begin{aligned} \frac{\partial \dot{T}}{\partial n_j} = & \frac{1}{\sum_{k=1}^{N_{\text{sp}}} [C]_k C_{p,k}} \left[ - \sum_{k=1}^{-1+N_{\text{sp}}} \left( H_k - \frac{W_k H_{N_{\text{sp}}}}{W_{N_{\text{sp}}}} \right) \frac{\partial \dot{\omega}_k}{\partial n_j} \right. \\ & \left. - \frac{1}{V} \frac{dT}{dt} (-C_{p,N_{\text{sp}}} + C_{p,j}) \right] \quad \text{for CONP,} \end{aligned} \quad (67a)$$

and:

$$\frac{\partial \dot{T}}{\partial n_j} = \frac{1}{\sum_{k=1}^{N_{\text{sp}}} [C]_k C_{v,k}} \left[ - \sum_{k=1}^{-1+N_{\text{sp}}} \left( U_k - \frac{W_k U_{N_{\text{sp}}}}{W_{N_{\text{sp}}}} \right) \frac{\partial \dot{\omega}_k}{\partial n_j} - \frac{1}{V} \frac{dT}{dt} (-C_{v,N_{\text{sp}}} + C_{v,j}) \right] \quad \text{for CONV.} \quad (67b)$$

Again, the derivative of the species production rate with respect to moles will be explored in Section 3.4.

### 3.2. State parameter source term derivatives

#### 3.2.1. Temperature derivative

The derivatives of the thermodynamic state parameter source terms with respect to temperature are given by differentiating Eq. (11):

$$\begin{aligned} \mathcal{J}_{2,1} &= \frac{\partial}{\partial T} \frac{dV}{dt} = \frac{\partial \dot{V}}{\partial T} \\ &= \frac{V}{[C]} \sum_{k=1}^{-1+N_{\text{sp}}} \left( 1 - \frac{W_k}{W_{N_{\text{sp}}}} \right) \left( \frac{\partial \dot{\omega}_k}{\partial T} + \frac{\dot{\omega}_k}{T} \right) \\ &\quad + \frac{V}{T} \left( \frac{d\dot{T}}{dT} - \frac{1}{T} \frac{dT}{dt} \right) \quad \text{for CONP,} \end{aligned} \quad (68a)$$

and:

$$\begin{aligned} \mathcal{J}_{2,1} &= \frac{\partial}{\partial T} \frac{dV}{dt} = \frac{\partial \dot{P}}{\partial T} \\ &= \mathcal{R} \sum_{k=1}^{-1+N_{\text{sp}}} \left( 1 - \frac{W_k}{W_{N_{\text{sp}}}} \right) \left( T \frac{\partial \dot{\omega}_k}{\partial T} + \dot{\omega}_k \right) \\ &\quad + \frac{P}{T} \left( \frac{d\dot{T}}{dT} - \frac{1}{T} \frac{dT}{dt} \right) \quad \text{for CONV.} \end{aligned} \quad (68b)$$

#### 3.2.2. State parameter derivative

Similarly, the derivatives of the thermodynamic state parameter source terms with respect to themselves are:

$$\mathcal{J}_{2,2} = \frac{\partial}{\partial V} \frac{dV}{dt} = \frac{\partial \dot{V}}{\partial V}$$



$$\begin{aligned}
&= \frac{1}{[C]} \sum_{k=1}^{-1+N_{\text{sp}}} \left(1 - \frac{W_k}{W_{N_{\text{sp}}}}\right) \left(V \frac{\partial \dot{\omega}_k}{\partial V} + \dot{\omega}_k\right) \\
&\quad + \frac{1}{T} \left(V \frac{d\dot{T}}{dV} + \dot{T}\right) \quad \text{for CONP,} \quad (69a)
\end{aligned}$$

and:

$$\begin{aligned}
\mathcal{J}_{2,2} &= \frac{\partial}{\partial P} \frac{dP}{dt} = \frac{\partial \dot{P}}{\partial P} \\
&= T\mathcal{R} \sum_{k=1}^{-1+N_{\text{sp}}} \left(1 - \frac{W_k}{W_{N_{\text{sp}}}}\right) \frac{\partial \dot{\omega}_k}{\partial P} \\
&\quad + \frac{1}{T} \left(P \frac{d\dot{T}}{dP} + \dot{T}\right) \quad \text{for CONV.} \quad (69b)
\end{aligned}$$

### 3.2.3. Molar derivative

Finally, the derivatives of the thermodynamic state parameter source terms with respect to the moles of species  $j$  are:

$$\begin{aligned}
\mathcal{J}_{2,j+2} &= \frac{\partial}{\partial n_j} \frac{dV}{dt} = \frac{\partial \dot{V}}{\partial n_j} \\
&= V \left( \frac{1}{[C]} \sum_{k=1}^{-1+N_{\text{sp}}} \left(1 - \frac{W_k}{W_{N_{\text{sp}}}}\right) \frac{\partial \dot{\omega}_k}{\partial n_j} + \frac{1}{T} \frac{d\dot{T}}{dn_j} \right) \quad \text{for CONP,} \quad (70a)
\end{aligned}$$

and:

$$\begin{aligned}
\mathcal{J}_{2,j+2} &= \frac{\partial}{\partial n_j} \frac{dV}{dt} = \frac{\partial \dot{V}}{\partial n_j} \\
&= \frac{P}{T} \frac{d\dot{T}}{dn_j} + T\mathcal{R} \sum_{k=1}^{-1+N_{\text{sp}}} \left(1 - \frac{W_k}{W_{N_{\text{sp}}}}\right) \frac{\partial \dot{\omega}_k}{\partial n_j} \quad \text{for CONV.} \quad (70b)
\end{aligned}$$

### 3.3. Molar source term derivatives

#### 3.3.1. Temperature derivative

The derivative of the net molar rate of production of a species  $k$  with respect to temperature is:

$$\mathcal{J}_{k+2,1} = \frac{\partial}{\partial T} \frac{dn_k}{dt} = \frac{\partial \dot{n}_k}{\partial T},$$

or:

$$\mathcal{J}_{k+2,1} = V \frac{\partial \dot{\omega}_k}{\partial T}. \quad (71)$$

### 3.3.2. State parameter derivatives

Similarly, the derivative of the net molar rate of production of a species  $k$  with respect to the state parameter is:

$$\begin{aligned}\mathcal{J}_{k+2,2} &= \frac{\partial}{\partial V} \frac{dn_k}{dt} = \frac{\partial \dot{n}_k}{\partial V} \\ &= V \frac{\partial \dot{\omega}_k}{\partial V} + \dot{\omega}_k\end{aligned}\quad \text{for CONP,} \quad (72a)$$

and:

$$\begin{aligned}\mathcal{J}_{k+2,2} &= \frac{\partial}{\partial P} \frac{dn_k}{dt} = \frac{\partial \dot{n}_k}{\partial P} \\ &= V \frac{\partial \dot{\omega}_k}{\partial P}\end{aligned}\quad \text{for CONV.} \quad (72b)$$

### 3.3.3. Molar derivative

Finally, the derivative of the net molar rate of production of a species  $k$  with respect to the moles of species  $j$  is:

$$\mathcal{J}_{k+2,j+2} = \frac{\partial}{\partial n_j} \frac{dn_k}{dt} = \frac{\partial \dot{n}_k}{\partial n_j},$$

or:

$$\mathcal{J}_{k+2,j+2} = V \frac{\partial \dot{\omega}_k}{\partial n_j}. \quad (73)$$

### 3.4. Species production rate derivatives

The derivatives of the net species production rate equation Eq. (18), with respect to temperature are:

$$\frac{\partial \dot{\omega}_k}{\partial T} = \sum_{i=1}^{N_{\text{reac}}} \left( \nu_{k,i} R_i \frac{\partial c_i}{\partial T} + \nu_{k,i} \frac{\partial R_i}{\partial T} c_i \right), \quad (74)$$

the state parameter:

$$\frac{\partial \dot{\omega}_k}{\partial V} = \sum_{i=1}^{N_{\text{reac}}} \left( \nu_{k,i} R_i \frac{\partial c_i}{\partial V} + \nu_{k,i} \frac{\partial R_i}{\partial V} c_i \right) \quad \text{for CONP,} \quad (75a)$$

$$\frac{\partial \dot{\omega}_k}{\partial P} = \sum_{i=1}^{N_{\text{reac}}} \left( \nu_{k,i} R_i \frac{\partial c_i}{\partial P} + \nu_{k,i} \frac{\partial R_i}{\partial P} c_i \right) \quad \text{for CONV,} \quad (75b)$$

and other species:

$$\frac{\partial \dot{\omega}_k}{\partial n_j} = \sum_{i=1}^{N_{\text{reac}}} \left( \nu_{k,i} R_i \frac{\partial c_i}{\partial n_j} + \nu_{k,i} \frac{\partial R_i}{\partial n_j} c_i \right). \quad (76)$$

### 3.5. Rate of progress derivatives

#### 3.5.1. Temperature derivative

Next, the rate of progress derivatives are evaluated, first with respect to temperature:

$$\frac{\partial R_i}{\partial T} = \frac{\partial}{\partial T} \left( k_{f,i} \prod_{k=1}^{N_{\text{sp}}} [C]_k^{\nu'_{k,i}} \right). \quad (77)$$

The derivative of the forward reaction rate coefficient is:

$$\frac{dk_{f,i}}{dT} = \frac{k_{f,i}}{T} \left( \beta_i + \frac{E_{ai}}{T\mathcal{R}} \right). \quad (78)$$

While evaluating derivatives for the Jacobian, it is important to expand terms—e.g., concentration, production rate, etc.—related to the last species to obtain the correct derivative, in this case using Eq. (12):

$$R_f = \left( \left( - \sum_{k=1}^{N_{\text{sp}}-1} [C]_k + \frac{P}{T\mathcal{R}} \right)^{\nu'_{N_{\text{sp}},i}} \right) k_{f,i} \prod_{k=1}^{N_{\text{sp}}-1} [C]_k^{\nu'_{k,i}}. \quad (79)$$

Hence, the full derivative of the forward rate of progress is:

$$\frac{\partial R_{f,i}}{\partial T} = \frac{dk_{f,i}}{dT} \prod_{k=1}^{N_{\text{sp}}} [C]_k^{\nu'_{k,i}} - \frac{[C] \nu'_{N_{\text{sp}},i}}{T} [C]_{N_{\text{sp}}}^{\nu'_{N_{\text{sp}},i}-1} k_{f,i} \prod_{k=1}^{N_{\text{sp}}-1} [C]_k^{\nu'_{k,i}}. \quad (80)$$

By defining a temporary variable  $S'_l$  (for species  $l = \{j, N_{\text{sp}}\}$ ):

$$S'_l = \nu'_{l,i} [C]_l^{\nu'_{l,i}-1} \prod_{\substack{1 \leq l \leq l-1 \\ l+1 \leq l \leq N_{\text{sp}}}} [C]_l^{\nu'_{l,i}}, \quad (81)$$

and using Eq. (78), Eq. (80) can be simplified to:

$$\frac{\partial R_{f,i}}{\partial T} = - \frac{[C] S'_{N_{\text{sp}}}}{T} k_{f,i} + \frac{R_{f,i}}{T} \left( \beta_i + \frac{E_{ai}}{T\mathcal{R}} \right). \quad (82)$$

Starting from Eq. (23) and applying the same expansion of the  $N_{\text{sp}}$ -th species' concentration as previously, the temperature derivative of the reverse rate of progress is:

$$\frac{\partial R_{r,i}}{\partial T} = \frac{dk_{r,i}}{dT} \prod_{k=1}^{N_{\text{sp}}} [C]_k^{\nu''_{k,i}} - \frac{[C] \nu''_{N_{\text{sp}},i}}{T} [C]_{N_{\text{sp}}}^{\nu''_{N_{\text{sp}},i}-1} k_{r,i} \prod_{k=1}^{N_{\text{sp}}-1} [C]_k^{\nu''_{k,i}}. \quad (83)$$

Next, Eq. (27) is considered to obtain the temperature derivative of the non-explicit reversible reaction rate coefficient:

$$\begin{aligned}\frac{dk_{r,i}}{dT} &= \left( -\frac{1}{K_{c,i}} \frac{dK_{c,i}}{dT} \frac{k_{f,i}}{K_{c,i}} + \frac{1}{K_{c,i}} \frac{dk_{f,i}}{dT} \right), \\ &= \left( -\frac{1}{K_{c,i}} \frac{dK_{c,i}}{dT} + \frac{1}{T} \left( \beta_i + \frac{E_{ai}}{T\mathcal{R}} \right) \right) k_{r,i}.\end{aligned}\quad (84)$$

The temperature derivative of the equilibrium constant is:

$$\frac{dK_{c,i}}{dT} = K_{c,i} \sum_{k=1}^{N_{\text{sp}}} \nu_{k,i} \frac{dB_k}{dT}, \quad (85)$$

with:

$$\frac{dB_k}{dT} = T \left( T \left( \frac{Ta_{k,4}}{5} + \frac{a_{k,3}}{4} \right) + \frac{a_{k,2}}{3} \right) + \frac{a_{k,1}}{2} + \frac{1}{T} \left( a_{k,0} - 1 + \frac{a_{k,5}}{T} \right), \quad (86)$$

giving:

$$\frac{dk_{r,i}}{dT} = \left( -\sum_{k=1}^{N_{\text{sp}}} \nu_{k,i} \frac{dB_k}{dT} + \frac{1}{T} \left( \beta_i + \frac{E_{ai}}{T\mathcal{R}} \right) \right) k_{r,i}. \quad (87)$$

Using a temporary value  $S''_{N_{\text{sp}}}$ —defined analogously to Eq. (81) for the reverse reaction rate—the full derivative of the reverse rate of progress with respect to temperature is obtained:

$$\frac{\partial R_{r,i}}{\partial T} = \left( -\sum_{k=1}^{N_{\text{sp}}} \nu_{k,i} \frac{dB_k}{dT} + \frac{1}{T} \left( \beta_i + \frac{E_{ai}}{T\mathcal{R}} \right) \right) R_{r,i} - \frac{[C]S''_{N_{\text{sp}}}}{T} k_{r,i}. \quad (88)$$

Finally, combining Eqs. (82) and (88) gives the total temperature derivative of the net rate of progress:

$$\begin{aligned}\frac{\partial R_i}{\partial T} &= \frac{R_{f,i}}{T} \left( \beta_i + \frac{E_{ai}}{T\mathcal{R}} \right) - \left( -\sum_{k=1}^{N_{\text{sp}}} \nu_{k,i} \frac{dB_k}{dT} + \frac{1}{T} \left( \beta_i + \frac{E_{ai}}{T\mathcal{R}} \right) \right) R_{r,i} \\ &\quad + \frac{[C]S''_{N_{\text{sp}}}}{T} k_{r,i} - \frac{[C]S'_{N_{\text{sp}}}}{T} k_{f,i}.\end{aligned}\quad (89)$$

### 3.5.2. State parameter derivatives

Following the outline of Section 3.5.1—while utilising Eq. (61) for the species concentration derivatives—the forward rate of progress derivatives are:

$$\frac{\partial R_{f,i}}{\partial V} = \frac{[C]S'_{N_{\text{sp}}}}{V}k_{f,i} - \frac{R_{f,i}}{V} \sum_{k=1}^{N_{\text{sp}}} \nu'_{k,i} \quad \text{for CONP,} \quad (90a)$$

$$\frac{\partial R_{f,i}}{\partial P} = \frac{S'_{N_{\text{sp}}}k_{f,i}}{T\mathcal{R}} \quad \text{for CONV.} \quad (90b)$$

Similarly, the reverse rate of progress derivatives are:

$$\frac{\partial R_{r,i}}{\partial V} = \frac{[C]S''_{N_{\text{sp}}}}{V}k_{r,i} - \frac{R_{r,i}}{V} \sum_{k=1}^{N_{\text{sp}}} \nu''_{k,i} \quad \text{for CONP,} \quad (91a)$$

and:

$$\frac{\partial R_{r,i}}{\partial P} = \frac{S''_{N_{\text{sp}}}k_{r,i}}{T\mathcal{R}} \quad \text{for CONV.} \quad (91b)$$

Combining Eqs. (90) and (91) gives:

$$\begin{aligned} \frac{\partial R_i}{\partial V} = \frac{1}{V} & \left( [C] \left( S'_{N_{\text{sp}}}k_{f,i} - S''_{N_{\text{sp}}}k_{r,i} \right) + \right. \\ & \left. \left( R_{r,i} \sum_{k=1}^{N_{\text{sp}}} \nu''_{k,i} - R_{f,i} \sum_{k=1}^{N_{\text{sp}}} \nu'_{k,i} \right) \right) \quad \text{for CONP,} \end{aligned} \quad (92a)$$

and:

$$\frac{\partial R_i}{\partial P} = \frac{1}{T\mathcal{R}} \left( S'_{N_{\text{sp}}}k_{f,i} - S''_{N_{\text{sp}}}k_{r,i} \right) \quad \text{for CONV.} \quad (92b)$$

### 3.5.3. Molar derivative

The derivative of the forward rate of progress with respect to the amount of moles of a species  $j$  is:

$$\frac{d}{dn_k} R_{f,i} = \left( \frac{\partial}{\partial n_j} \prod_{k=1}^{N_{\text{sp}}} [C]^{\nu'_{k,i}} \right) k_{f,i} . \quad (93)$$

Combining Eqs. (65) and (93) the molar derivative of the forward rate of progress is:

$$\frac{\partial R_{f,i}}{\partial n_j} = k_{f,i} \sum_{k=1}^{N_{\text{sp}}} \left( -\frac{\delta_{N_{\text{sp}}k}}{V} + \frac{\delta_{jk}}{V} \right) \nu'_{k,i} [C]_k^{\nu'_{k,i}-1} \prod_{\substack{1 \leq l \leq k-1 \\ k+1 \leq l \leq N_{\text{sp}}}} [C]_l^{\nu'_{l,i}} \quad (94)$$

with the same temporary variables  $S'_j$  and  $S'_{N_{\text{sp}}}$  as defined previously, this can be simplified to:

$$\frac{\partial R_{f,i}}{\partial n_j} = \frac{k_{f,i}}{V} \left( -S'_{N_{\text{sp}}} + S'_j \right) . \quad (95)$$

By the same process, the reverse rate of progress derivative is calculated as:

$$\frac{\partial R_{r,i}}{\partial n_j} = \frac{k_{r,i}}{V} \left( -S''_{N_{\text{sp}}} + S''_j \right) , \quad (96)$$

and from Eqs. (95) and (96) the net rate of progress molar derivative is found:

$$\frac{\partial R_i}{\partial n_j} = -\frac{k_{r,i}}{V} \left( -S''_{N_{\text{sp}}} + S''_j \right) + \frac{k_{f,i}}{V} \left( -S'_{N_{\text{sp}}} + S'_j \right) . \quad (97)$$

#### 3.5.4. Pressure-dependent reactions

The P-Log and Chebyshev pressure-dependent reactions, described by Eqs. (46) and (47) require separate treatment from the derivatives of strictly Arrhenius-based reaction rate formulations examined in Sections 3.5.1 to 3.5.3. Beginning with P-Log reactions, the derivative of the forward rate coefficient with respect to temperature is:

$$\begin{aligned} \frac{\partial k_{f,i}}{\partial T} = & \left( \frac{1}{k_1} \frac{dk_1}{dT} + \frac{1}{-\log(P_1) + \log(P_2)} \left( -\frac{1}{k_1} \frac{dk_1}{dT} + \frac{1}{k_2} \frac{dk_2}{dT} \right) \times \left( \right. \\ & \left. -\log(P_1) + \log(P) \right) \right) k_{f,i} , \end{aligned} \quad (98)$$

and the derivatives of  $k_1$  and  $k_2$  are given by Eq. (78) with the corresponding Arrhenius parameters (see Eqs. (44) and (45)) substituted in.

Simplifying Eq. (98) gives:

$$\frac{\partial k_{f,i}}{\partial T} = \frac{k_{f,i}}{T} \left( \frac{(-\log(P_1) + \log(P))}{-\log(P_1) + \log(P_2)} \times \right.$$

$$\left(-\beta_1 + \beta_2 - \frac{E_{a_1}}{T\mathcal{R}} + \frac{E_{a_2}}{T\mathcal{R}}\right) + \beta_1 + \frac{E_{a_1}}{T\mathcal{R}} \Bigg) . \quad (99)$$

Similar to Section 3.5.1, Eq. (99) may be substituted into Eqs. (80) and (83) to give:

$$\begin{aligned} \frac{\partial R_i}{\partial T} = & \left( \frac{(-\log(P_1) + \log(P)) \left(-\beta_1 + \beta_2 - \frac{E_{a_1}}{T\mathcal{R}} + \frac{E_{a_2}}{T\mathcal{R}}\right)}{-\log(P_1) + \log(P_2)} + \beta_1 + \frac{E_{a_1}}{T\mathcal{R}} \right) \times \\ & \left( \frac{R_{f,i} - R_{r,i}}{T} \right) + R_{r,i} \sum_{k=1}^{N_{\text{sp}}} \nu_{k,i} \frac{dB_k}{dT} + \frac{[C]}{T} \left( S''_{N_{\text{sp}}} k_{r,i} - S'_{N_{\text{sp}}} k_{f,i} \right) . \end{aligned} \quad (100)$$

For CONV problems, the P-Log forward reaction rate coefficient is also a function of the pressure:

$$\frac{\partial k_{f,i}}{\partial P} = \frac{(-\log(k_1) + \log(k_2)) k_{f,i}}{P(-\log(P_1) + \log(P_2))} , \quad (101)$$

substituting this into the net rate of progress derivative gives:

$$\begin{aligned} \frac{\partial R_i}{\partial P} = & \frac{1}{T\mathcal{R}} \left( -S''_{N_{\text{sp}}} k_{r,i} + S'_{N_{\text{sp}}} k_{f,i} \right) + \\ & \frac{(-\log(k_1) + \log(k_2)) (R_{f,i} - R_{r,i})}{P(-\log(P_1) + \log(P_2))} \quad \text{for CONV.} \end{aligned} \quad (102)$$

Next, the temperature derivative of Chebyshev reactions will be considered:

$$\frac{\partial k_{f,i}}{\partial T} = \log(10) k_{f,i} \sum_{\substack{1 \leq l \leq N_P \\ 1 \leq j \leq N_T}} \frac{d\tilde{T}}{dT} (j-1) \mathcal{T}_{l-1}(\tilde{P}) U_{j-2}(\tilde{T}) \eta_{l,j} , \quad (103)$$

where  $U_n$  is the Chebyshev polynomial of the second kind of degree  $n$ , expressed as:

$$U_n(x) = \frac{\sin((n+1) \arccos x)}{\sin(\arccos x)} \quad (104)$$

and:

$$\frac{d\tilde{T}}{dT} = \frac{-2}{T^2 \left( -\frac{1}{T_{\min}} + \frac{1}{T_{\max}} \right)} , \quad (105)$$

giving:

$$\frac{\partial k_{f,i}}{\partial T} = \log(10) k_{f,i} \sum_{\substack{1 \leq l \leq N_P \\ 1 \leq j \leq N_T}} - \frac{2 \mathcal{T}_{l-1}(\tilde{P}) U_{j-2}(\tilde{T}) \eta_{l,j}}{T^2 \left( -\frac{1}{T_{\min}} + \frac{1}{T_{\max}} \right)} (j-1) . \quad (106)$$

Following the same process for Arrhenius-based reactions (see Section 3.5.1), the derivative of the net rate of progress with respect to temperature is:

$$\begin{aligned} \frac{\partial R_i}{\partial T} = & \sum_{\substack{1 \leq l \leq N_P \\ 1 \leq j \leq N_T}} \left[ - \frac{2 \log(10) \mathcal{T}_{l-1}(\tilde{P}) U_{j-2}(\tilde{T}) \eta_{l,j}}{T^2 \left( -\frac{1}{T_{\min}} + \frac{1}{T_{\max}} \right)} (j-1) \right] (R_{f,i} - R_{r,i}) + \\ & \sum_{k=1}^{N_{\text{sp}}} \nu_{k,i} \frac{dB_k}{dT} R_{r,i} + \frac{[C]}{T} \left( S''_{N_{\text{sp}}} k_{r,i} - S'_{N_{\text{sp}}} k_{f,i} \right) . \end{aligned} \quad (107)$$

For CONV problems, the derivative of the forward rate coefficient with respect to pressure must again be considered:

$$\frac{\partial k_{f,i}}{\partial P} = \log(10) k_{f,i} \sum_{\substack{1 \leq l \leq N_P \\ 1 \leq j \leq N_T}} \frac{d\tilde{P}}{dP} (l-1) \mathcal{T}_{j-1}(\tilde{T}) U_{l-2}(\tilde{P}) \eta_{l,j} , \quad (108)$$

with:

$$\frac{d\tilde{P}}{dP} = \frac{2}{P (\log(P_{\max}) - \log(P_{\min}))} , \quad (109)$$

giving:

$$\frac{\partial k_{f,i}}{\partial P} = \log(10) k_{f,i} \sum_{\substack{1 \leq l \leq N_P \\ 1 \leq j \leq N_T}} \frac{2(l-1) \mathcal{T}_{j-1}(\tilde{T}) U_{l-2}(\tilde{P}) \eta_{l,j}}{P (\log(P_{\max}) - \log(P_{\min}))} . \quad (110)$$

Finally, the net rate of progress derivative for a Chebyshev reaction with respect to pressure is:

$$\begin{aligned} \frac{\partial R_i}{\partial P} = & \log(10) (R_{f,i} - R_{r,i}) \times \\ & \sum_{\substack{1 \leq l \leq N_P \\ 1 \leq j \leq N_T}} \frac{2(l-1) \mathcal{T}_{j-1}(\tilde{T}) U_{l-2}(\tilde{P}) \eta_{l,j}}{P (\log(P_{\max}) - \log(P_{\min}))} + \\ & \frac{1}{T\mathcal{R}} \left( -S''_{N_{\text{sp}}} k_{r,i} + S'_{N_{\text{sp}}} k_{f,i} \right) \quad \text{for CONV.} \end{aligned} \quad (111)$$



### 3.6. Pressure modification/Falloff function derivatives

#### 3.6.1. Elementary reactions

For elementary reactions, the derivative of the pressure-modification term with respect to temperature is:

$$\frac{\partial c_i}{\partial T} = 0, \quad (112)$$

and with respect to the state parameter:

$$\frac{\partial c_i}{\partial V} = 0 \quad \text{for CONP}, \quad (113a)$$

$$\frac{\partial c_i}{\partial P} = 0 \quad \text{for CONV}, \quad (113b)$$

and finally, with respect to the moles of species  $j$ :

$$\frac{\partial c_i}{\partial n_j} = 0. \quad (114)$$

#### 3.6.2. Third-body enhanced reactions

For a **mixture** based third-body enhanced reaction Eq. (34) is differentiated with respect to temperature to give:

$$\frac{\partial [X]_i}{\partial T} = -\frac{[C]\alpha_{N_{sp},i}}{T}, \quad (115)$$

and with respect to the state parameter:

$$\frac{\partial [X]_i}{\partial V} = \frac{1}{V} \left( [C]\alpha_{N_{sp},i} - [X]_i \right) \quad \text{for CONP}, \quad (116a)$$

$$\frac{\partial [X]_i}{\partial P} = \frac{\alpha_{N_{sp},i}}{T\mathcal{R}} \quad \text{for CONV}, \quad (116b)$$

and finally, with respect to the moles of species  $j$ :

$$\frac{\partial [X]_i}{\partial n_j} = \frac{1}{V} \left( -\alpha_{N_{sp},i} + \alpha_{j,i} \right). \quad (117)$$

If  $\alpha_{j,i} = 1$  for all species  $j$  (i.e., a **unity** third-body), Eqs. (115) to (117) may be simplified to:

$$\frac{\partial c_i}{\partial T} = -\frac{[C]}{T}, \quad (118)$$

and for the state parameter:

$$\frac{\partial c_i}{\partial V} = 0 \quad \text{for CONP,} \quad (119a)$$

$$\frac{\partial c_i}{\partial P} = \frac{1}{T\mathcal{R}} \quad \text{for CONV,} \quad (119b)$$

and finally for the moles of species  $j$ :

$$\frac{\partial c_i}{\partial n_j} = 0 \quad . \quad (120)$$

If the third-body is the  $m$ th **species**, Eqs. (115) to (117) become:

$$\frac{\partial c_i}{\partial T} = -\frac{\delta_{N_{\text{sp}}m}}{T} [C] \quad , \quad (121)$$

and:

$$\frac{\partial c_i}{\partial V} = \frac{\delta_{N_{\text{sp}}m}}{V} ([C] - [C]_{N_{\text{sp}}}) + \frac{[C]_m}{V} (\delta_{N_{\text{sp}}m} - 1) \quad \text{for CONP,} \quad (122a)$$

$$\frac{\partial c_i}{\partial P} = \frac{\delta_{N_{\text{sp}}m}}{T\mathcal{R}} \quad \text{for CONV,} \quad (122b)$$

and for the molar derivative:

$$\frac{\partial c_i}{\partial n_j} = \frac{1}{V} (-\delta_{N_{\text{sp}}m} + \delta_{jm}) \quad . \quad (123)$$

### 3.6.3. Unimolecular/ recombination fall-off reactions

Derivatives of the third-body pressure modification term for unimolecular/ recombination fall-off reactions—given by Eq. (24)—are quite involved, and will be broken up over the next sections. The derivative of full third-body pressure modification term for fall-off reactions will be given in this section, while Section 3.6.4 will provide the same derivatives for chemically-activated bimolecular reactions. Subsequently, the derivatives of the reduced pressure and falloff blending factors will be explored in Sections 3.6.5 and 3.6.6 respectively.

The derivatives of the unimolecular/ recombination fall-off reaction third-body pressure modification term are:

$$\frac{\partial c_i}{\partial T} = \frac{1}{P_{r,i} + 1} \left( P_{r,i} \frac{\partial F_i}{\partial T} + \frac{\partial P_{r,i}}{\partial T} (F_i - c_i) \right) \quad , \quad (124)$$

and with respect to the state parameter:

$$\frac{\partial c_i}{\partial V} = \frac{1}{P_{r,i} + 1} \left( P_{r,i} \frac{\partial F_i}{\partial V} + \frac{\partial P_{r,i}}{\partial V} (F_i - c_i) \right) \quad \text{for CONP,} \quad (125a)$$

$$\frac{\partial c_i}{\partial P} = \frac{1}{P_{r,i} + 1} \left( P_{r,i} \frac{\partial F_i}{\partial P} + \frac{\partial P_{r,i}}{\partial P} (F_i - c_i) \right) \quad \text{for CONV,} \quad (125b)$$

and finally the molar derivative:

$$\frac{\partial c_i}{\partial n_j} = \frac{1}{P_{r,i} + 1} \left( P_{r,i} \frac{\partial F_i}{\partial n[j]} + \frac{\partial P_{r,i}}{\partial n_j} (F_i - c_i) \right) \quad . \quad (126)$$

#### 3.6.4. Chemically-activated bimolecular reactions

Similarly, the chemically-activated bimolecular reactions are as follows:

$$\frac{\partial c_i}{\partial T} = \frac{1}{P_{r,i} + 1} \left( \frac{\partial F_i}{\partial T} - \frac{\partial P_{r,i}}{\partial T} c_i \right) \quad , \quad (127)$$

$$(128)$$

and for the state parameter derivative:

$$\frac{\partial c_i}{\partial V} = \frac{1}{P_{r,i} + 1} \left( \frac{\partial F_i}{\partial V} - \frac{\partial P_{r,i}}{\partial V} c_i \right) \quad \text{for CONP,} \quad (129a)$$

$$\frac{\partial c_i}{\partial P} = \frac{1}{P_{r,i} + 1} \left( \frac{\partial F_i}{\partial P} - \frac{\partial P_{r,i}}{\partial P} c_i \right) \quad \text{for CONV,} \quad (129b)$$

and finally, the molar derivative:

$$\frac{\partial c_i}{\partial n_j} = \frac{1}{P_{r,i} + 1} \left( \frac{\partial F_i}{\partial n_j} - \frac{\partial P_{r,i}}{\partial n_j} c_i \right) \quad . \quad (130)$$

#### 3.6.5. Reduced pressure

Next the reduced pressure derivatives in Eqs. (124) to (129) will be evaluated; these depend on the form of the third-body efficiency used in Eq. (38), thus we will first work out the derivatives for each third-body efficiency form, and then develop a generalized form for compact representation. For a third-body concentration based upon the entire mixture, (i.e., Eq. (34)) the temperature derivative is:

$$\frac{\partial P_{r,i}}{\partial T} = \frac{P_{r,i}}{T} \left( \beta_0 - \beta_\infty + \frac{E_{a,0}}{T\mathcal{R}} - \frac{E_{a,\infty}}{T\mathcal{R}} \right) - \frac{[C]k_{0,i}\alpha_{N_{sp},i}}{Tk_{\infty,i}} \quad , \quad (131)$$

and the state parameter derivatives are:

$$\frac{\partial P_{r,i}}{\partial V} = -\frac{P_{r,i}}{V} + \frac{[C]k_{0,i}\alpha_{N_{sp},i}}{Vk_{\infty,i}} \quad \text{for CONP, (132a)}$$

$$\frac{\partial P_{r,i}}{\partial P} = \frac{k_{0,i}\alpha_{N_{sp},i}}{Tk_{\infty,i}\mathcal{R}} \quad \text{for CONV, (132b)}$$

and finally, the molar derivative is given by:

$$\frac{\partial P_{r,i}}{\partial n_j} = \frac{k_{0,i}(-\alpha_{N_{sp},i} + \alpha_{j,i})}{k_{\infty,i}V} \quad . \quad (133)$$

For a unity third-body concentration (i.e., all  $\alpha_{k,i} = 1$ ):

$$\frac{\partial P_{r,i}}{\partial T} = \frac{P_{r,i}}{T} \left( \beta_0 - \beta_\infty - 1 + \frac{E_{a,0}}{T\mathcal{R}} - \frac{E_{a,\infty}}{T\mathcal{R}} \right) \quad , \quad (134)$$

and the state parameter derivatives are:

$$\frac{\partial P_{r,i}}{\partial V} = 0 \quad \text{for CONP, (135a)}$$

$$\frac{\partial P_{r,i}}{\partial P} = \frac{k_{0,i}}{k_{\infty,i}} \frac{1}{\mathcal{R}T} \quad \text{for CONV, (135b)}$$

and the molar derivative is:

$$\frac{\partial P_{r,i}}{\partial n_j} = 0 \quad . \quad (136)$$

Finally, for species-based third-body (i.e., the species  $m$  alone acts as the third body):

$$\frac{\partial P_{r,i}}{\partial T} = \frac{P_{r,i}}{T} \left( \beta_0 - \beta_\infty + \frac{E_{a,0}}{T\mathcal{R}} - \frac{E_{a,\infty}}{T\mathcal{R}} \right) - \frac{[C]k_{0,i}\delta_{N_{sp}m}}{Tk_{\infty,i}} \quad , \quad (137)$$

for the state parameter derivative:

$$\frac{\partial P_{r,i}}{\partial V} = -\frac{P_{r,i}}{V} + \frac{[C]k_{0,i}\delta_{N_{sp}m}}{Vk_{\infty,i}} \quad \text{for CONP, (138a)}$$

$$\frac{\partial P_{r,i}}{\partial P} = \frac{k_{0,i}\delta_{N_{sp}m}}{Tk_{\infty,i}\mathcal{R}} \quad \text{for CONV, (138b)}$$

and the molar derivative:

$$\frac{\partial P_{r,i}}{\partial n_j} = \frac{k_{0,i}}{V k_{\infty,i}} \left( -\delta_{N_{\text{sp}}m} + \delta_{jm} \right) \quad . \quad (139)$$

Equations (131) to (138) may be recast in a more generalized form using temporary variables  $\Theta_{P_{r,i},\partial\ldots}$  and  $\bar{\theta}_{P_{r,i},\partial\ldots}$ —where, for example,  $\Theta_{P_{r,i},\partial T}$  corresponds to part of the reduced-pressure derivative with respect to temperature—to replace terms in each individual form of the reduced-pressure derivatives:

$$\frac{\partial P_{r,i}}{\partial T} = P_{r,i} \Theta_{P_{r,i},\partial T} + \bar{\theta}_{P_{r,i},\partial T} \quad , \quad (140)$$

and the state parameter:

$$\frac{\partial P_{r,i}}{\partial V} = P_{r,i} \Theta_{P_{r,i},\partial V} + \bar{\theta}_{P_{r,i},\partial V} \quad \text{for CONP}, \quad (141a)$$

$$\frac{\partial P_{r,i}}{\partial P} = \bar{\theta}_{P_{r,i},\partial P} \quad \text{for CONV}, \quad (141b)$$

and the molar derivative:

$$\frac{\partial P_{r,i}}{\partial n_j} = \frac{k_{0,i} \bar{\theta}_{P_{r,i},\partial n_j}}{V k_{\infty,i}} \quad . \quad (142)$$

with:

$$\Theta_{P_{r,i},\partial T} = \begin{cases} \frac{1}{T} \left( \beta_0 - \beta_\infty + \frac{E_{a,0}}{T\mathcal{R}} - \frac{E_{a,\infty}}{T\mathcal{R}} \right) & \text{if mix,} \\ \frac{1}{T} \left( \beta_0 - \beta_\infty - 1 + \frac{E_{a,0}}{T\mathcal{R}} - \frac{E_{a,\infty}}{T\mathcal{R}} \right) & \text{if unity,} \\ \frac{1}{T} \left( \beta_0 - \beta_\infty + \frac{E_{a,0}}{T\mathcal{R}} - \frac{E_{a,\infty}}{T\mathcal{R}} \right) & \text{if species,} \end{cases} \quad (143)$$

$$\bar{\theta}_{P_{r,i},\partial T} = \begin{cases} -\frac{[C] k_{0,i} \alpha_{N_{\text{sp}},i}}{T k_{\infty,i}} & \text{if mix,} \\ 0 & \text{if unity,} \\ -\frac{[C] k_{0,i} \delta_{N_{\text{sp}}m}}{T k_{\infty,i}} & \text{if species,} \end{cases} \quad (144)$$

$$\Theta_{P_{r,i},\partial V} = \begin{cases} -\frac{1}{V} & \text{if mix,} \\ 0 & \text{if unity,} \\ -\frac{1}{V} & \text{if species,} \end{cases} \quad (145)$$

$$\bar{\theta}_{P_r,i,\partial V} = \begin{cases} \frac{[C]k_{0,i}\alpha_{N_{sp},i}}{Vk_{\infty,i}} & \text{if mix,} \\ 0 & \text{if unity,} \\ \frac{[C]k_{0,i}\delta_{N_{sp}m}}{Vk_{\infty,i}} & \text{if species,} \end{cases} \quad (146)$$

$$\bar{\theta}_{P_r,i,\partial P} = \begin{cases} \frac{k_{0,i}\alpha_{N_{sp},i}}{Tk_{\infty,i}\mathcal{R}} & \text{if mix,} \\ \frac{k_{0,i}}{Tk_{\infty,i}\mathcal{R}} & \text{if unity,} \\ \frac{k_{0,i}\delta_{N_{sp}m}}{Tk_{\infty,i}\mathcal{R}} & \text{if species,} \end{cases} \quad (147)$$

$$\bar{\theta}_{P_r,i,\partial n_j} = \begin{cases} -\alpha_{N_{sp},i} + \alpha_{j,i} & \text{if mix,} \\ 0 & \text{if unity,} \\ -\delta_{N_{sp}m} + \delta_{jm} & \text{if species.} \end{cases} \quad (148)$$

### 3.6.6. Falloff blending factor

Derivatives of the falloff blending factor—except for all but the Lindemann falloff blending factor, which is not a function of the reduced pressure—rely upon the reduced pressure derivatives developed in Section 3.6.5. First, the blending factor for each falloff reaction type will be differentiated along with any subcomponents (e.g., the  $F_{cent}$  term for Troe falloff reactions). Next, the reduced pressured derivatives given by Eqs. (140) to (142) will be substituted in and finally a generalized form for the falloff blending factor derivatives will be determined.

For Lindemann falloff reactions:

$$\frac{\partial F_i}{\partial T} = 0, \quad (149)$$

$$(150)$$

and, for the state parameter:

$$\frac{\partial F_i}{\partial V} = 0 \quad \text{for CONP,} \quad (151a)$$

$$\frac{\partial F_i}{\partial P} = 0 \quad \text{for CONV,} \quad (151b)$$

and the molar derivative:

$$\frac{\partial F_i}{\partial n_j} = 0. \quad (152)$$

For Troe falloff reactions:

$$\frac{\partial F_i}{\partial T} = \frac{\partial F_i}{\partial F_{cent}} \frac{dF_{cent}}{dT} + \frac{\partial F_i}{\partial P_{r,i}} \frac{\partial P_{r,i}}{\partial T} \quad , \quad (153)$$

and the state parameter derivative:

$$\frac{\partial F_i}{\partial V} = \frac{\partial F_i}{\partial P_{r,i}} \frac{\partial P_{r,i}}{\partial V} \quad \text{for CONP}, \quad (154a)$$

$$\frac{\partial F_i}{\partial P} = \frac{\partial F_i}{\partial P_{r,i}} \frac{\partial P_{r,i}}{\partial P} \quad \text{for CONV}, \quad (154b)$$

and:

$$\frac{\partial F_i}{\partial n_j} = \frac{\partial F_i}{\partial P_{r,i}} \frac{\partial P_{r,i}}{\partial n_j} \quad . \quad (155)$$

The Troe falloff blending factor derivative with respect to  $F_{cent}$  is:

$$\frac{\partial F_i}{\partial F_{cent}} = \frac{F_i}{\frac{A_{Tro}^2}{B_{Tro}^2} + 1} \left( \frac{2A_{Tro} \log(F_{cent})}{B_{Tro}^2 \left( \frac{A_{Tro}^2}{B_{Tro}^2} + 1 \right)} \left( \frac{A_{Tro}}{B_{Tro}} \frac{\partial B_{Tro}}{\partial F_{cent}} - \frac{\partial A_{Tro}}{\partial F_{cent}} \right) + \frac{1}{F_{cent}} \right) \quad , \quad (156)$$

and:

$$\frac{dF_{cent}}{dT} = \frac{a}{T^*} \exp\left(-\frac{T}{T^*}\right) - \frac{\exp\left(-\frac{T}{T^{***}}\right)}{T^{***}} (-a + 1) + \frac{T^{**}}{T^2} \exp\left(-\frac{T^{**}}{T}\right) \quad , \quad (157)$$

and:

$$\frac{\partial F_i}{\partial P_{r,i}} = \frac{2F_i A_{Tro} \log(F_{cent})}{B_{Tro}^2 \left( \frac{A_{Tro}^2}{B_{Tro}^2} + 1 \right)^2} \left( \frac{A_{Tro}}{B_{Tro}} \frac{\partial B_{Tro}}{\partial P_{r,i}} - \frac{\partial A_{Tro}}{\partial P_{r,i}} \right) \quad . \quad (158)$$

Finally, the derivatives of  $A_{Tro}$  and  $B_{Tro}$  are:

$$\frac{\partial A_{Tro}}{\partial F_{cent}} = -\frac{0.67}{F_{cent} \log(10)} \quad , \quad (159)$$

$$\frac{\partial B_{Troee}}{\partial F_{cent}} = -\frac{1.1762}{F_{cent} \log(10)} \quad , \quad (160)$$

$$\frac{\partial A_{Troee}}{\partial P_{r,i}} = \frac{1}{P_{r,i} \log(10)} \quad , \quad (161)$$

and:

$$\frac{\partial B_{Troee}}{\partial P_{r,i}} = -\frac{0.14}{P_{r,i} \log(10)} \quad . \quad (162)$$

$$(163)$$

Combining Eqs. (159) to (162) with Eqs. (156) and (158) yields:

$$\frac{\partial F_i}{\partial F_{cent}} = -\frac{F_i B_{Troee}}{F_{cent} (A_{Troee}^2 + B_{Troee}^2) \log(10)} (2A_{Troee} (1.1762A_{Troee} - 0.67B_{Troee}) \log(F_{cent}) - B_{Troee} (A_{Troee}^2 + B_{Troee}^2) \log(10)) \quad , \quad (164)$$

and:

$$\frac{\partial F_i}{\partial P_{r,i}} = -\frac{2F_i A_{Troee} \left( \frac{0.14A_{Troee}}{B_{Troee}} + 1 \right) \log(F_{cent})}{B_{Troee}^2 P_{r,i} \left( \frac{A_{Troee}^2}{B_{Troee}^2} + 1 \right)^2 \log(10)} \quad (165)$$

Equations (157), (164) and (165) can then be substituted into Eqs. (153) to (155) to obtain a final form for the Troe-falloff blending function derivatives, which will be given as a generalized form at the end of this section.

For SRI falloff reactions, the temperature derivative of the falloff blending factor is:

$$\begin{aligned} \frac{\partial F_i}{\partial T} = F_i & \left( \frac{X \left( -\frac{\exp(-\frac{T}{c})}{c} + \frac{ab}{T^2} \exp\left(-\frac{b}{T}\right) \right)}{a \exp\left(-\frac{b}{T}\right) + \exp\left(-\frac{T}{c}\right)} + \right. \\ & \left. \frac{\partial P_{r,i}}{\partial T} \frac{dX}{dP_{r,i}} \log \left[ \right. \right. \\ & \left. \left. a \exp\left(-\frac{b}{T}\right) + \exp\left(-\frac{T}{c}\right) \right] + \frac{e}{T} \right) \quad , \quad (166) \end{aligned}$$



and the state parameter derivatives:

$$\frac{\partial F_i}{\partial V} = F_i \frac{\partial P_{r,i}}{\partial V} \frac{dX}{dP_{r,i}} \log \left( a \exp \left( -\frac{b}{T} \right) + \exp \left( -\frac{T}{c} \right) \right) \quad \text{for CONP,} \quad (167a)$$

$$\frac{\partial F_i}{\partial P} = F_i \frac{\partial P_{r,i}}{\partial P} \frac{dX}{dP_{r,i}} \log \left( a \exp \left( -\frac{b}{T} \right) + \exp \left( -\frac{T}{c} \right) \right) \quad \text{for CONV,} \quad (167b)$$

and finally, with respect to species moles:

$$\frac{\partial F_i}{\partial n_j} = F_i \frac{\partial P_{r,i}}{\partial n_j} \frac{dX}{dP_{r,i}} \log \left( a \exp \left( -\frac{b}{T} \right) + \exp \left( -\frac{T}{c} \right) \right) \quad . \quad (168)$$

The derivatives of the SRI exponent  $X$  are:

$$\frac{dX}{dP_{r,i}} = -\frac{2X^2 \log(P_{r,i})}{P_{r,i} \log^2(10)} \quad , \quad (169)$$

$$\frac{\partial X}{\partial n_j} = \frac{\partial P_{r,i}}{\partial n_j} \frac{dX}{dP_{r,i}} \quad . \quad (170)$$

As with the reduced-pressure derivatives, Eqs. (149), (151) to (155) and (166) to (168) may be represented in a general form via introduction of temporary variables  $\Theta_{F_i, \partial \dots}$ , giving for the temperature derivative:

$$\frac{\partial F_i}{\partial T} = F_i \Theta_{F_i, \partial T} \quad , \quad (171)$$

for the state parameter derivatives:

$$\frac{\partial F_i}{\partial V} = F_i \Theta_{F_i, \partial V} \quad \text{for CONP,} \quad (172a)$$

$$\frac{\partial F_i}{\partial P} = F_i \Theta_{F_i, \partial P} \quad \text{for CONV,} \quad (172b)$$

and finally, for the molar derivative:

$$\frac{\partial F_i}{\partial n_j} = \frac{F_i k_{0,i} \Theta_{F_i, \partial n_j}}{V k_{\infty,i}} \bar{\theta}_{P_{r,i}, \partial n_j} \quad . \quad (173)$$

For Lindemann falloff reactions:

$$\Theta_{F_i, \partial T} = 0 \quad , \quad (174)$$

and, for the state parameter derivatives:

$$\Theta_{F_i, \partial V} = 0 \quad , \quad (175a)$$

$$\Theta_{F_i, \partial P} = 0 \quad , \quad (175b)$$

and for the molar derivative:

$$\Theta_{F_i, \partial n_j} = 0 \quad . \quad (176)$$

For Troe falloff reactions:

$$\begin{aligned} \Theta_{F_i, \partial T} = & -\frac{B_{Troe}}{F_{cent} P_{r,i} (A_{Troe}^2 + B_{Troe}^2) \log(10)} \times \left( \right. \\ & 2A_{Troe} F_{cent} (0.14A_{Troe} + B_{Troe}) \times \\ & \left( P_{r,i} \Theta_{P_{r,i}, \partial T} + \bar{\theta}_{P_{r,i}, \partial T} \right) \log(F_{cent}) + P_{r,i} \frac{dF_{cent}}{dT} \times \left( \right. \\ & 2A_{Troe} (1.1762A_{Troe} - 0.67B_{Troe}) \log(F_{cent}) - \\ & \left. \left. B_{Troe} (A_{Troe}^2 + B_{Troe}^2) \log(10) \right) \right) \quad , \quad (177) \end{aligned}$$

and for the state parameter derivatives:

$$\Theta_{F_i, \partial V} = -\frac{2A_{Troe} B_{Troe} \log(F_{cent})}{P_{r,i} (A_{Troe}^2 + B_{Troe}^2) \log(10)} \times \left( \right. \\ \left. 0.14A_{Troe} + B_{Troe} \right) \left( P_{r,i} \Theta_{P_{r,i}, \partial V} + \bar{\theta}_{P_{r,i}, \partial V} \right) \quad , \quad (178a)$$

$$\Theta_{F_i, \partial P} = -\frac{2A_{Troe} B_{Troe} \bar{\theta}_{P_{r,i}, \partial P} (0.14A_{Troe} + B_{Troe}) \log(F_{cent})}{P_{r,i} (A_{Troe}^2 + B_{Troe}^2) \log(10)} \quad , \quad (178b)$$

and the molar derivative:

$$\Theta_{F_i, \partial n_j} = -\frac{2A_{Troe} B_{Troe} (0.14A_{Troe} + B_{Troe}) \log(F_{cent})}{P_{r,i} (A_{Troe}^2 + B_{Troe}^2) \log(10)} \quad . \quad (179)$$

where  $\Theta_{P_{r,i}, \partial \dots}$  and  $\bar{\theta}_{P_{r,i}, \partial \dots}$  are given by Eqs. (143) to (148) respectively.

Finally, for SRI falloff reactions:

$$\Theta_{F_i, \partial T} = -\frac{X \left( \frac{\exp(-\frac{T}{c})}{c} - \frac{ab}{T^2} \exp\left(-\frac{b}{T}\right) \right)}{a \exp\left(-\frac{b}{T}\right) + \exp\left(-\frac{T}{c}\right)} + \frac{e}{T} - \left( \right.$$

$$\frac{2X^2 \log \left( a \exp \left( -\frac{b}{T} \right) + \exp \left( -\frac{T}{c} \right) \right)}{P_{r,i} \log^2 (10)} \times \left( P_{r,i} \Theta_{P_{r,i}, \partial T} + \bar{\theta}_{P_{r,i}, \partial T} \right) \log (P_{r,i}) \quad , \quad (180)$$

and:

$$\Theta_{F_i, \partial V} = -\frac{2X^2 \log (P_{r,i})}{P_{r,i} \log^2 (10)} \left( P_{r,i} \Theta_{P_{r,i}, \partial V} + \bar{\theta}_{P_{r,i}, \partial V} \right) \log \left( \left( a \exp \left( \frac{T}{c} \right) + \exp \left( \frac{b}{T} \right) \right) \exp \left( -\frac{T}{c} - \frac{b}{T} \right) \right) \quad , \quad (181a)$$

$$\Theta_{F_i, \partial P} = -\frac{2X^2 \bar{\theta}_{P_{r,i}, \partial P} \log (P_{r,i})}{P_{r,i} \log^2 (10)} \log \left( a \exp \left( -\frac{b}{T} \right) + \exp \left( -\frac{T}{c} \right) \right) \quad , \quad (181b)$$

and finally, for the molar derivative:

$$\Theta_{F_i, \partial n_j} = -\frac{2X^2 \log \left( a \exp \left( -\frac{b}{T} \right) + \exp \left( -\frac{T}{c} \right) \right)}{P_{r,i} \log^2 (10)} \log (P_{r,i}) \quad . \quad (182)$$

### 3.6.7. Unimolecular/ recombination fall-off reactions (temporary product form)

Using the temporary products developed in Sections 3.6.5 and 3.6.6, the fall-off reaction derivatives developed in Eqs. (124) to (126) may be simplified to:

$$\frac{\partial c_i}{\partial T} = \frac{F_i \bar{\theta}_{P_{r,i}, \partial T}}{P_{r,i} + 1} + \left( -\frac{P_{r,i} \Theta_{P_{r,i}, \partial T}}{P_{r,i} + 1} + \Theta_{F_i, \partial T} + \Theta_{P_{r,i}, \partial T} - \frac{\bar{\theta}_{P_{r,i}, \partial T}}{P_{r,i} + 1} \right) c_i \quad , \quad (183)$$

and, for the state parameter derivatives:

$$\frac{\partial c_i}{\partial V} = \frac{F_i \bar{\theta}_{P_{r,i}, \partial V}}{P_{r,i} + 1} + \left( -\frac{P_{r,i} \Theta_{P_{r,i}, \partial V}}{P_{r,i} + 1} + \Theta_{F_i, \partial V} + \Theta_{P_{r,i}, \partial V} - \frac{\bar{\theta}_{P_{r,i}, \partial V}}{P_{r,i} + 1} \right) c_i \quad \text{for CONP,} \quad (184a)$$

$$\frac{\partial c_i}{\partial P} = \frac{F_i \bar{\theta}_{P_{r,i}, \partial P}}{P_{r,i} + 1} + \left( \Theta_{F_i, \partial P} - \frac{\bar{\theta}_{P_{r,i}, \partial P}}{P_{r,i} + 1} \right) c_i \quad \text{for CONV,} \quad (184b)$$

and the molar derivative:

$$\frac{\partial c_i}{\partial n_j} = \frac{k_{0,i} \bar{\theta}_{P_{r,i}, \partial n_j}}{V k_{\infty,i} (P_{r,i} + 1)} \left( F_i (P_{r,i} \Theta_{F_i, \partial n_j} + 1) - c_i \right) \quad . \quad (185)$$

The temporary products in Eqs. (183) to (185) are given by Eqs. (143) to (148) and Eqs. (174) to (182).

### 3.6.8. Chemically-activated bimolecular reactions (temporary product form)

Similarly, the chemically-activated reaction derivatives in Eqs. (127), (129) and (130) may be written as:

$$\frac{\partial c_i}{\partial T} = \left( -\frac{P_{r,i} \Theta_{P_{r,i}, \partial T}}{P_{r,i} + 1} + \Theta_{F_i, \partial T} - \frac{\bar{\theta}_{P_{r,i}, \partial T}}{P_{r,i} + 1} \right) c_i \quad , \quad (186)$$

and the state parameter derivatives:

$$\frac{\partial c_i}{\partial V} = \left( -\frac{P_{r,i} \Theta_{P_{r,i}, \partial V}}{P_{r,i} + 1} + \Theta_{F_i, \partial V} - \frac{\bar{\theta}_{P_{r,i}, \partial V}}{P_{r,i} + 1} \right) c_i \quad \text{for CONP} \quad (187a)$$

$$\frac{\partial c_i}{\partial P} = \left( \Theta_{F_i, \partial P} - \frac{\bar{\theta}_{P_{r,i}, \partial P}}{P_{r,i} + 1} \right) c_i \quad \text{for CONV} \quad (187b)$$

and the molar derivative:

$$\frac{\partial c_i}{\partial n_j} = \frac{k_{0,i} \bar{\theta}_{P_{r,i}, \partial n_j} (F_i \Theta_{F_i, \partial n_j} - c_i)}{k_{\infty,i} V (P_{r,i} + 1)} \quad . \quad (188)$$

The temporary products are the same as those detailed in Section 3.6.7.

## 4. Final jacobian form

Here we give a summary of the Jacobian derivations in the previous sections, as a complete reference guide to the equations evaluated by `pyJac`.

### 4.1. Temperature derivatives

In this section, the derivatives of all source terms with respect to the temperature are considered.

#### 4.1.1. Temperature source term derivatives

Starting from Eq. (59), Eq. (71) is substituted in to yield:

$$\begin{aligned} \mathcal{J}_{1,1} = & \frac{1}{\sum_{k=1}^{N_{\text{sp}}} [C]_k C_{p,k}} \left[ \frac{dT}{dt} \sum_{k=1}^{N_{\text{sp}}} \left( -\frac{dC_{p,k}}{dT} + \frac{C_{p,N_{\text{sp}}}}{T} \right) [C]_k + \right. \\ & \sum_{k=1}^{N_{\text{sp}}-1} \left( \left( -H_k + \frac{W_k H_{N_{\text{sp}}}}{W_{N_{\text{sp}}}} \right) \frac{\mathcal{J}_{k+2,1}}{V} + \right. \\ & \left. \left. \left( -C_{p,k} + \frac{W_k C_{p,k}}{W_{N_{\text{sp}}}} \right) \dot{\omega}_k \right) \right] \end{aligned} \quad \text{for CONP,} \quad (189a)$$

and similarly:

$$\begin{aligned} \mathcal{J}_{1,1} = & \frac{1}{\sum_{k=1}^{N_{\text{sp}}} [C]_k C_{v,k}} \left[ \frac{dT}{dt} \sum_{k=1}^{N_{\text{sp}}} \left( -\frac{dC_{v,k}}{dT} + \frac{C_{v,N_{\text{sp}}}}{T} \right) [C]_k + \right. \\ & \sum_{k=1}^{N_{\text{sp}}-1} \left( \left( -U_k + \frac{W_k U_{N_{\text{sp}}}}{W_{N_{\text{sp}}}} \right) \frac{\mathcal{J}_{k+2,1}}{V} + \right. \\ & \left. \left. \left( -C_{v,k} + \frac{W_k C_{v,N_{\text{sp}}}}{W_{N_{\text{sp}}}} \right) \dot{\omega}_k \right) \right] \end{aligned} \quad \text{for CONV.} \quad (189b)$$

#### 4.1.2. State parameter source term derivatives

Similarly, Eqs. (52) and (71) are substituted into Eq. (68), giving:

$$\begin{aligned} \mathcal{J}_{2,1} = & \frac{\partial}{\partial T} \frac{dV}{dt} = \frac{\partial \dot{V}}{\partial T} \\ = & \frac{V}{[C]} \sum_{k=1}^{N_{\text{sp}}-1} \left( 1 - \frac{W_k}{W_{N_{\text{sp}}}} \right) \left( \frac{\mathcal{J}_{k+2,1}}{V} + \frac{\dot{\omega}_k}{T} \right) \\ & + \frac{V}{T} \left( \mathcal{J}_{1,1} - \frac{1}{T} \frac{dT}{dt} \right) \end{aligned} \quad \text{for CONP,} \quad (190a)$$

and:

$$\mathcal{J}_{2,1} = \frac{\partial}{\partial T} \frac{dV}{dt} = \frac{\partial \dot{P}}{\partial T}$$

$$\begin{aligned}
&= \mathcal{R} \sum_{k=1}^{N_{\text{sp}}-1} \left( 1 - \frac{W_k}{W_{N_{\text{sp}}}} \right) \left( T \frac{\mathcal{J}_{k+2,1}}{V} + \dot{\omega}_k \right) \\
&\quad + \frac{P}{T} \left( \mathcal{J}_{1,1} - \frac{1}{T} \frac{dT}{dt} \right) \quad \text{for CONV.} \quad (190b)
\end{aligned}$$

#### 4.1.3. Molar source term derivatives

From Eq. (71) and Eq. (74), a general form for the molar source term derivative with respect to temperature is obtained:

$$\mathcal{J}_{k+2,1} = V \sum_{i=1}^{N_{\text{reac}}} \left( \nu_{k,i} R_i \frac{\partial c_i}{\partial T} + \nu_{k,i} \frac{\partial R_i}{\partial T} c_i \right), \quad (191)$$

where the rate of progress derivatives are given by Eqs. (89), (100) and (107) for arrhenius-based—i.e., elementary, third-body and falloff/chemically-activated—reactions, P-Log reactions and Chebyshev reactions respectively. The temperature derivatives of the pressure modification term are found in Eqs. (115), (118) and (121) for third-body reactions, and Eqs. (183) and (186) for falloff/chemically-activated reactions respectively.

#### 4.2. State parameter derivatives

In this section, the derivatives of all source terms with respect to the state parameter are considered.

##### 4.2.1. Temperature source term derivatives

Similar to Section 4.1.1, Eq. (72) is substituted into Eq. (62) to yield:

$$\begin{aligned}
\mathcal{J}_{1,2} = \frac{1}{\sum_{k=1}^{N_{\text{sp}}} V[C]_k C_{p,k}} &\left[ \right. \\
&- \sum_{k=1}^{N_{\text{sp}}-1} \left( H_k - \frac{W_k H_{N_{\text{sp}}}}{W_{N_{\text{sp}}}} \right) (\mathcal{J}_{k+2,2} - \dot{\omega}_k) + \\
&\left. \frac{dT}{dt} \sum_{k=1}^{N_{\text{sp}}-1} (-C_{p,N_{\text{sp}}} + C_{p,k}) [C]_k \right] \quad \text{for CONP,} \quad (192a)
\end{aligned}$$

$$\begin{aligned}
\mathcal{J}_{1,2} = \frac{1}{\sum_{k=1}^{N_{\text{sp}}} [C]_k C_{v,k}} &\left[ \right. \\
&- \sum_{k=1}^{N_{\text{sp}}-1} \left( U_k - \frac{W_k U_{N_{\text{sp}}}}{W_{N_{\text{sp}}}} \right) \frac{\mathcal{J}_{k+2,2}}{V} -
\end{aligned}$$

$$\left. \frac{C_{v,N_{\text{sp}}}}{T\mathcal{R}} \frac{dT}{dt} \right] \quad \text{for CONV.} \quad (192b)$$

#### 4.2.2. State parameter source term derivatives

Next, Eq. (69) is simplified via Eqs. (60) and (72) to give:

$$\begin{aligned} \mathcal{J}_{2,2} = & \frac{1}{[C]} \sum_{k=1}^{N_{\text{sp}}-1} \left( 1 - \frac{W_k}{W_{N_{\text{sp}}}} \right) \mathcal{J}_{k+2,2} \\ & + \frac{1}{T} (V \mathcal{J}_{1,2} + \dot{T}) \end{aligned} \quad \text{for CONP,} \quad (193a)$$

and:

$$\begin{aligned} \mathcal{J}_{2,2} = & \frac{T\mathcal{R}}{V} \sum_{k=1}^{N_{\text{sp}}-1} \left( 1 - \frac{W_k}{W_{N_{\text{sp}}}} \right) \mathcal{J}_{k+2,2} \\ & + \frac{1}{T} (P \mathcal{J}_{1,2} + \dot{T}) \end{aligned} \quad \text{for CONV.} \quad (193b)$$

#### 4.2.3. Molar source term derivatives

To obtain a final form for the molar source term derivative with respect to the state parameter, Eqs. (72) and (75) are combined:

$$\mathcal{J}_{k+2,2} = V \sum_{i=1}^{N_{\text{reac}}} \left( \nu_{k,i} R_i \frac{\partial c_i}{\partial V} + \nu_{k,i} \frac{\partial R_i}{\partial V} c_i \right) + \dot{\omega}_k \quad \text{for CONP,} \quad (194a)$$

$$\mathcal{J}_{k+2,2} = V \sum_{i=1}^{N_{\text{reac}}} \left( \nu_{k,i} R_i \frac{\partial c_i}{\partial P} + \nu_{k,i} \frac{\partial R_i}{\partial P} c_i \right) \quad \text{for CONV.} \quad (194b)$$

The derivative of the net rate of progress with respect to the state parameter is given by Eq. (92) for arrhenius-based reactions. For P-Log and Chebyshev reactions in a CONV system Eqs. (102) and (111) are used, while Eq. (92) is used for a CONP system. The pressure modification term derivatives are given by Eqs. (116), (119) and (122) for third-body enhanced reactions, and Eqs. (184) and (187) for falloff/chemically-activated reactions respectively.

#### 4.3. Molar derivatives

Finally, this section details the Jacobian entries corresponding to derivatives with respect to the species moles.

#### 4.3.1. Temperature source term derivatives

The temperature source term derivative with respect to the moles of species  $j$ , Eq. (67), is combined with Eq. (73), giving:

$$\mathcal{J}_{1,j+2} = \frac{1}{\sum_{k=1}^{N_{\text{sp}}} V[C]_k C_{p,k}} \left[ \begin{aligned} & - \sum_{k=1}^{N_{\text{sp}}-1} \left( H_k - \frac{W_k H_{N_{\text{sp}}}}{W_{N_{\text{sp}}}} \right) \mathcal{J}_{k+2,j+2} \\ & - \frac{dT}{dt} (-C_{p,N_{\text{sp}}} + C_{p,j}) \end{aligned} \right] \quad \text{for CONP,} \quad (195a)$$

and:

$$\mathcal{J}_{1,j+2} = \frac{1}{\sum_{k=1}^{N_{\text{sp}}} V[C]_k C_{v,k}} \left[ \begin{aligned} & - \sum_{k=1}^{N_{\text{sp}}-1} \left( U_k - \frac{W_k U_{N_{\text{sp}}}}{W_{N_{\text{sp}}}} \right) \mathcal{J}_{k+2,j+2} \\ & - \frac{dT}{dt} (-C_{v,N_{\text{sp}}} + C_{v,j}) \end{aligned} \right] \quad \text{for CONV.} \quad (195b)$$

#### 4.3.2. State parameter derivatives

From Eqs. (63), (70) and (73), the final form of the state parameter source term derivative with respect to the moles of species  $j$  is:

$$\mathcal{J}_{2,j+2} = \frac{1}{[C]} \sum_{k=1}^{N_{\text{sp}}-1} \left( 1 - \frac{W_k}{W_{N_{\text{sp}}}} \right) \mathcal{J}_{k+2,j+2} + \frac{V}{T} \mathcal{J}_{1,j+2} \quad \text{for CONP,} \quad (196a)$$

and:

$$\mathcal{J}_{2,j+2} = \frac{T\mathcal{R}}{V} \sum_{k=1}^{N_{\text{sp}}-1} \left( 1 - \frac{W_k}{W_{N_{\text{sp}}}} \right) \mathcal{J}_{k+2,j+2} + \frac{P}{T} \mathcal{J}_{2,j+2} \quad \text{for CONV.} \quad (196b)$$

#### 4.3.3. Molar source term derivatives

Finally, Eqs. (73) and (76) are combined yielding:

$$\mathcal{J}_{k+2,j+2} = V \sum_{i=1}^{N_{\text{reac}}} \left( \nu_{k,i} R_i \frac{\partial c_i}{\partial n_j} + \nu_{k,i} \frac{\partial R_i}{\partial n_j} c_i \right) . \quad (197)$$



As `pyJac` evaluates these derivative entries by looping over the reactions  $i$  in the model, Eq. (197) is converted to an update form:

$$\mathcal{J}_{k+2,j+2} += V \left( \nu_{k,i} R_i \frac{\partial c_i}{\partial n_j} + \nu_{k,i} \frac{\partial R_i}{\partial n_j} c_i \right) \quad k = 1, \dots, N_{\text{sp}} - 1 \quad (198)$$

The molar derivatives of the net rate of progress are given by Eq. (97), and the pressure modification term by Eqs. (117), (120) and (123) for third-body enhanced reactions, and Eqs. (185) and (188) for falloff/chemically-activated reactions, respectively.

## 5. References

- [1] A. Meurer, C. P. Smith, M. Paprocki, O. Čertík, S. B. Kirpichev, M. Rocklin, A. Kumar, S. Ivanov, J. K. Moore, S. Singh, T. Rathnayake, S. Vig, B. E. Granger, R. P. Muller, F. Bonazzi, H. Gupta, S. Vats, F. Johansson, F. Pedregosa, M. J. Curry, A. R. Terrel, v. Roučka, A. Saboo, I. Fernando, S. Kulal, R. Cimrman, A. Scopatz, Sympy: symbolic computing in python, *PeerJ Computer Science* 3 (2017) e103. [doi:10.7717/peerj-cs.103](https://doi.org/10.7717/peerj-cs.103).
- [2] S. R. Turns, *An Introduction to Combustion: Concepts and Applications*, 3rd Edition, McGraw-Hill, New York, 2012.
- [3] S. Gordon, B. J. McBride, Computer program for calculation of complex chemical equilibrium compositions and applications, Vol. 1, National Aeronautics and Space Administration, Office of Management, Scientific and Technical Information Program, 1994.
- [4] T. Lu, C. K. Law, Toward accommodating realistic fuel chemistry in large-scale computations, *Prog. Energy Comb. Sci.* 35 (2) (2009) 192–215. [doi:10.1016/j.pecs.2008.10.002](https://doi.org/10.1016/j.pecs.2008.10.002).
- [5] D. G. Goodwin, H. K. Moffat, R. L. Speth, Cantera: An object-oriented software toolkit for chemical kinetics, thermodynamics, and transport processes, <http://www.cantera.org>, version 2.3.0 (2017). [doi:10.5281/zenodo.170284](https://doi.org/10.5281/zenodo.170284).
- [6] F. A. Lindemann, S. Arrhenius, I. Langmuir, N. R. Dhar, J. Perrin, W. C. McC Lewis, Discussion on “the radiation theory of chemical action”, *Trans. Faraday Soc.* 17 (1922) 598–606. [doi:10.1039/TF9221700598](https://doi.org/10.1039/TF9221700598).
- [7] R. G. Gilbert, K. Luther, J. Troe, Theory of thermal unimolecular reactions in the fall-off range. II. Weak collision rate constants, *Ber. Bunsenges. Phys. Chem.* 87 (2) (1983) 169–177. [doi:10.1002/bbpc.19830870218](https://doi.org/10.1002/bbpc.19830870218).
- [8] P. H. Stewart, C. W. Larson, D. M. Golden, Pressure and temperature dependence of reactions proceeding via a bound complex. 2. Application to  $2\text{CH}_3 \rightarrow \text{C}_2\text{H}_5 + \text{H}$ , *Combust. Flame* 75 (1) (1989) 25–31. [doi:10.1016/0010-2180\(89\)90084-9](https://doi.org/10.1016/0010-2180(89)90084-9).

- [9] Reaction Design: San Diego, [CHEMKIN-PRO 15113](#) (2012).  
URL <http://www.ansys.com/Products/Fluids/ANSYS-Chemkin-Pro>
- [10] P. K. Venkatesh, A. M. Dean, M. H. Cohen, R. W. Carr, Chebyshev expansions and sensitivity analysis for approximating the temperature- and pressure-dependence of chemically-activated reactions, *Rev. Chem. Eng.* 13 (1) (1997) 1–67. [doi:10.1515/REVCE.1997.13.1.1](#).
- [11] P. K. Venkatesh, A. Y. Chang, A. M. Dean, M. H. Cohen, R. W. Carr, Parameterization of pressure- and temperature-dependent kinetics in multiple well reactions, *AIChE J.* 43 (5) (1997) 1331–1340. [doi:10.1002/aic.690430522](#).
- [12] P. K. Venkatesh, Damped pseudospectral functional forms of the falloff behavior of unimolecular reactions, *J. Phys. Chem. A* 104 (2) (2000) 280–287. [doi:10.1021/jp991458u](#).
